# Supplementary material for: MAGIC: Detecting Advanced Persistent Threats via Masked Graph Representation Learning
Source: arXiv:2310.09831 source file (2023-10-15)
Supplement: Supplementary file 1 [file appendix.tex]

\appendix

\section{Detailed Graph Construction Steps}\label{appe_a}

\noindent\textbf{Noise Reduction.} \emph{Noise reduction} is used in various recent works\cite{aptlearnbasedatlas-11,aptlearnbasedshadewatcher-18,aptlearnbasedthreatrace-17,aptlearnbasedprovgem-15} to reduce the complexity of provenance graphs and remove redundant and useless information. \system{} applies a mild noise reduction approach as \system{} is less sensitive to the scale of the provenance graph and more information is preserved in this way. Given a pair of nodes, \system{} remove all redundant edges \emph{of the same type} between them. Compared with noise reduction done in recent works\cite{aptlearnbasedatlas-11,aptlearnbasedshadewatcher-18}, we neither delete irrelevant nodes nor merge nodes with same semantics. This is because (1) attack-irrelevant nodes provides information for benign system behaviors and (2) multiple nodes with same semantics duplicate the information propagated to near-by nodes and impact on their embeddings.

\noindent\textbf{Attribute Extraction.} Provenance graphs used in \system{} have both attributed nodes and edges. Different formats of audit logs describe system entities and interactions in different ways. For simple log formats, attributes can be directly obtained from entity and interaction labels. For sophisticated log formats, \system{} leverages \emph{multi-label hashing}(i.e. xxhash\cite{xxhash-27}) to convert detailed description of system entities and interactions into labels.

\noindent\textbf{Constructing Graph Feature.} During this procedure, attributes of nodes and edges are encoded into one-hot form. However, the provenance graph is still inconsistent at this time, as multiple types of edges may exist between the same pair of nodes. In this case, all edges between a pair of nodes are merged into a new edge, whose one-hot encoding is calculated as the sum of the one-hot encodings of the original edges.

\section{Time and Space Complexity of \system{}}\label{appe_b}
Given a piece of audit logs with $N$ system entities and $E$ system interactions, the graph construction steps builds a provenance graph in $O(N+E)$ time, masked feature reconstruction is completed in $O(N+E)$ time and sample-based structure reconstruction takes only $O(N)$ time. Training of the detection module takes $O(NlogN)$ time to build a K-D Tree and memorize benign embeddings and detection result of a single target is obtained in $O(logN)$ time. Thus, the overall time complexity of \system{} during training and inference is $O(NlogN+E)$, which is linear to the size of audit logs.

\system{}'s memory consumption largely depends on the number of raw graph features \emph{t} and its embedding dimension \emph{d}. The graph representation module takes up $O((N+E)*t)$ space to store a provenance graph and $O((N+E)*d)$ space to generate graph embeddings. The detection module takes $O(N*d)$ space to memorize benign embeddings. The overall space complexity of \system{} is $O((N+E)*(t+d))$, preventing out-of-memory(OOM) problems on huge datasets.

\section{Targeted Attack and Countermeasure: An Example}\label{appe_c}
\system{} models an entity's behavior through information propagation and aggregation in its multi-hop neighborhood. Based on this fact, attackers may realize that abnormal behaviors can be covered up by breaking the causal relationship between two malicious entities into numerous sequentially connected benign interactions, so that those two entities do not appear in each other's multi-hop neighborhood. While this is a common flaw of GNN-based detectors, we claim that such infiltration can be avoided through more complicated provenance graph construction. An easy solution to this is to establish causal relationships between system entities with meta-paths, which brings entities remote yet connected in certain patterns to one-hop distance.
\section{Auto-encoder Based Anomaly Detection}\label{appe_d}
Among traditional applications of machine learning, anomaly detection via auto-encoders is common practice. Typically, auto-encoders are trained to reconstructing a target and minimize its reconstruction loss. Thus, the reconstruction loss of a newly-arrived sample indicates how similar it behaves to training samples and samples with high reconstruction error are detected as outliers. However, we do not apply auto-encoder based outlier detection based on two reasons: (1) our sample-based structure reconstruction produces high-variance reconstruction loss on single sample, which prevents stable threshold-based outlier detection and (2) \system{} performs batched log level detection by detecting outliers in system state embeddings, which do not have a reconstruction target and cannot be compared in reconstruction error.
