# Supplementary material for: MAGIC: Detecting Advanced Persistent Threats via Masked Graph Representation Learning
Source: arXiv:2310.09831 source file (2023-10-15)
Supplement: Supplementary file 2 [file appendix_revised.tex]

\appendix

\section{Analysis on Adversarial Attack}\label{appe_a_revised}
Adversarial attacks such as evasion attacks and poison attacks are tricky to implement but still possible to carry out. Two types of adversarial attacks are potentially practical against \system{}, manipulating input audit logs or exploiting model architecture. The later approach is not an option for \system{}'s attackers, as they have no access to \system{}'s inner parameters. Similar to SIGL~\cite{aptlearnbasedsigl-58}, we conduct a simple experiment concerning \system{}'s robustness against graph manipulations, which shows these attacks do not affect \system{}'s detection effectiveness. 

In this experiment, we expect attackers have no knowledge of \system{}'s inner parameters and cannot get any feedback from \system{}. However, attackers can freely manipulate the malicious entities within \system{}'s input audit logs, as well as a small proportion of benign entities. Consequently, we consider four types of attacks:

\textbf{Malicious Feature Evasion (MFE).} Attackers have altered the features of all malicious entities in the raw audit logs trying to evade detection. This affects the node initial embeddings of the input provenance graph and forces malicious entities to mimic benign ones in node features.

\textbf{Malicious Structure Evasion (MSE).} Attackers have adding new edges between malicious entities and benign ones, so that malicious entities behave more normally and tend to have local structures more similar to benign entities. This affects the graph representation module and pull the embeddings of malicious nodes towards benign ones, making them more difficult to identify.

\textbf{Combined Evasion (MCE).} This type of attack is a combination of the MFE and MSE and causes malicious entities to approximate benign ones in both features and structures.

\textbf{Benign Feature Poison (BFP).} Attackers have manipulated the features of entities to poison \system{}. Attackers injected some benign entities with similar initial features as malicious entities, trying to convince \system{} that the malicious entities behave normally. This shifts benign entities to mimic malicious ones in node features, gradually poisons \system{}'s detection module.

We evaluated \system{}'s robustness against the above four attack strategies on the Trace dataset and we present the results in Table~\ref{tab_adversarial}. Experimental results confirms that \system{} is robust enough against adversarial attacks. MFE has almost no impact on \system{}'s effectiveness. \system{} is slightly more vulnerable facing the structure evasion attacks, because the graph structure is critical to unsupervised graph representation learning. However, the structure attacks still have little impact on \system{}'s detection effectiveness. We believe that the feature and structure reconstruction involved in our graph representation module contributes to this robustness, as it learns a model to reconstruct both node features and its neighboring structure with the information from its neighbors. Consequently, adversarial attacks involving feature and structure altering of malicious entities will fail, and with \system{}'s model itself well-protected, attackers have to either extend their effort on searching and manipulating benign entities, or find other attack strategies against \system{}. Meanwhile, BFP has a relatively greater impact on \system{}'s performance. However, under BFP, only 0.057 AUC reduction is achieved by manipulating the input feature of an enormous 161,029 benign entities. This level of interference in the benign system is beyond the capability of ordinary attackers. Consequently, an effective BFP attack is also very difficult to carry out.

\begin{table}[t]
\centering
\small
\setlength{\belowcaptionskip}{0.2cm}
\caption{Impact of different adversarial attack strategies on \system{}'s detection effectiveness.}
\label{tab_adversarial_letter}
\begin{tabular}{|c|c|c|c|c|c|}
\hline
Attack Type & None & MFE & MSE & MCE & BFP \\
\hline

AUC & 0.9999 & 0.9999 & 0.9999 & 0.9994 & 0.9942\\
\hline
\end{tabular}
\end{table}

\section{Time and Space Complexity of \system{}}\label{appe_b_revised}

Given number of system entities $N$, number of system interactions $E$, initial embedding dimension \emph{t}, graph representation dimension $d$, number of GAT layers $l$ and mask rate $r$ the graph construction steps builds a featured provenance graph in $O((N+E) * t)$ time, masked feature reconstruction is completed in $O((N+E) * d^2 * l * r)$ time and sample-based structure reconstruction takes only $O(N * d)$ time. Training of the detection module takes $O(N *logN * d)$ time to build a K-D Tree and memorize benign embeddings. Detection result of a single target is obtained in $O(logN * d * k)$ time. Thus, the overall time complexity of \system{} during training and inference is $O(N*logN * d * k+E * d ^2 * l * r + (N + E) * t)$.

\system{}'s memory consumption largely depends on $d$ and $t$. The graph representation module takes up $O((N+E)*t)$ space to store a provenance graph and $O((N+E)*(t +d))$ space to generate output embeddings. The detection module takes $O(N*d)$ space to memorize benign embeddings. The overall space complexity of \system{} is $O((N+E)*(t+d))$.

\section{Hyper-parameter Choice Guideline }\label{appe_f_revised}

For most hyper-parameters involved in \system{}, including $l$ and $r$, default choices works fine in all conditions. \system{}'s users may just select $l$ equals 2 or 3 and $r$ equals 0.5 in all applications. For the embedding dimension $d$, the choice is up to the user himself, as a higher $d$ results in better performance at the cost of resource consumption.

The choice of detection threshold $\theta$ depends on the corresponding dataset \system{} is operating on. However, \textcolor{blue}{finding a precise $\theta$ is not necessary on each individual dataset, according to Sec.~\ref{sec_evaluation_5_revised}. Even if there is only benign data available, users may adjust and choose the optimal $\theta$ according to the resulting false positive rate (i.e. use the first $\theta$ when false positive rate is below the desired value). Here we provide a simple analysis on how wide is the threshold selection range and what consequence selecting different $\theta$ may lead to.}

\noindent\textcolor{blue}{\textbf{Impact of Different $\theta$ Choices.} Altering $\theta$ does not lead to drastic changes in detection results, especially for \#FN. For example, on the DARPA E3 Trace dataset, changing $\theta$ from 1000 to 5000 results in 2 more FNs and an 1\% decrease in FPR. On the E3 THEIA dataset, altering $\theta$ from 100 to 500 provides 0.5\% FPR decrease and does not change \#FN. On the CADETS dataset, setting $\theta$ as 100 instead of 10 leads to a 10\% decreased FPR with only 30 new FNs generated.}

\noindent\textcolor{blue}{\textbf{Quantifing the Threshold Selection Range.} By limiting FPR below 1\% on entity level tasks, we get a minimum $\theta$ equals 1980 on Trace dataset, 180 on THEIA dataset and 95 on CADETS dataset. The resulting recall is respectively 0.99985, 0.99996 and 0.99782. Meanwhile, the maximum $\theta$ that ensures recall > 99\% is actually 6600, 1020 and 120 on the three different datasets. The space between the minimum and maximum $\theta$ is big enough and the curves are flat. Consequently, MAGIC doesn't need a precise $\theta$ to obtain the desirable result and selecting threshold $\theta$ based on false positive rate is practical.}

\section{Noise Reduction}\label{appe_c_revised}

\emph{Noise reduction} is used in various recent works~\cite{aptlearnbasedatlas-11,aptlearnbasedshadewatcher-18,aptlearnbasedthreatrace-17,aptlearnbasedprovgem-15} to reduce the complexity of provenance graphs and remove redundant and useless information. \system{} applies a mild noise reduction approach as \system{} is less sensitive to the scale of the provenance graph and more information is preserved in this way. Compared with noise reduction done in recent works~\cite{aptlearnbasedatlas-11,aptlearnbasedshadewatcher-18}, we neither delete irrelevant nodes nor merge nodes with same semantics. This is because (1) attack-irrelevant nodes provides information for benign system behaviors and (2) multiple nodes with same semantics duplicate the information propagated to near-by nodes and impact on their embeddings.

\section{Auto-encoder Based Anomaly Detection}\label{appe_d_revised}
Among traditional applications of machine learning, anomaly detection via auto-encoders is common practice. Typically, auto-encoders are trained to reconstructing a target and minimize its reconstruction loss. Thus, the reconstruction loss of a newly-arrived sample indicates how similar it behaves to training samples and samples with high reconstruction error are detected as outliers. However, we do not apply auto-encoder based outlier detection based on two reasons: (1) our sample-based structure reconstruction produces high-variance reconstruction loss on single sample, which prevents stable threshold-based outlier detection and (2) \system{} performs batched log level detection by detecting outliers in system state embeddings, which do not have a reconstruction target and cannot be compared in reconstruction error.

\begin{figure}[t]
    \centering
    \includegraphics[width=0.46\textwidth]{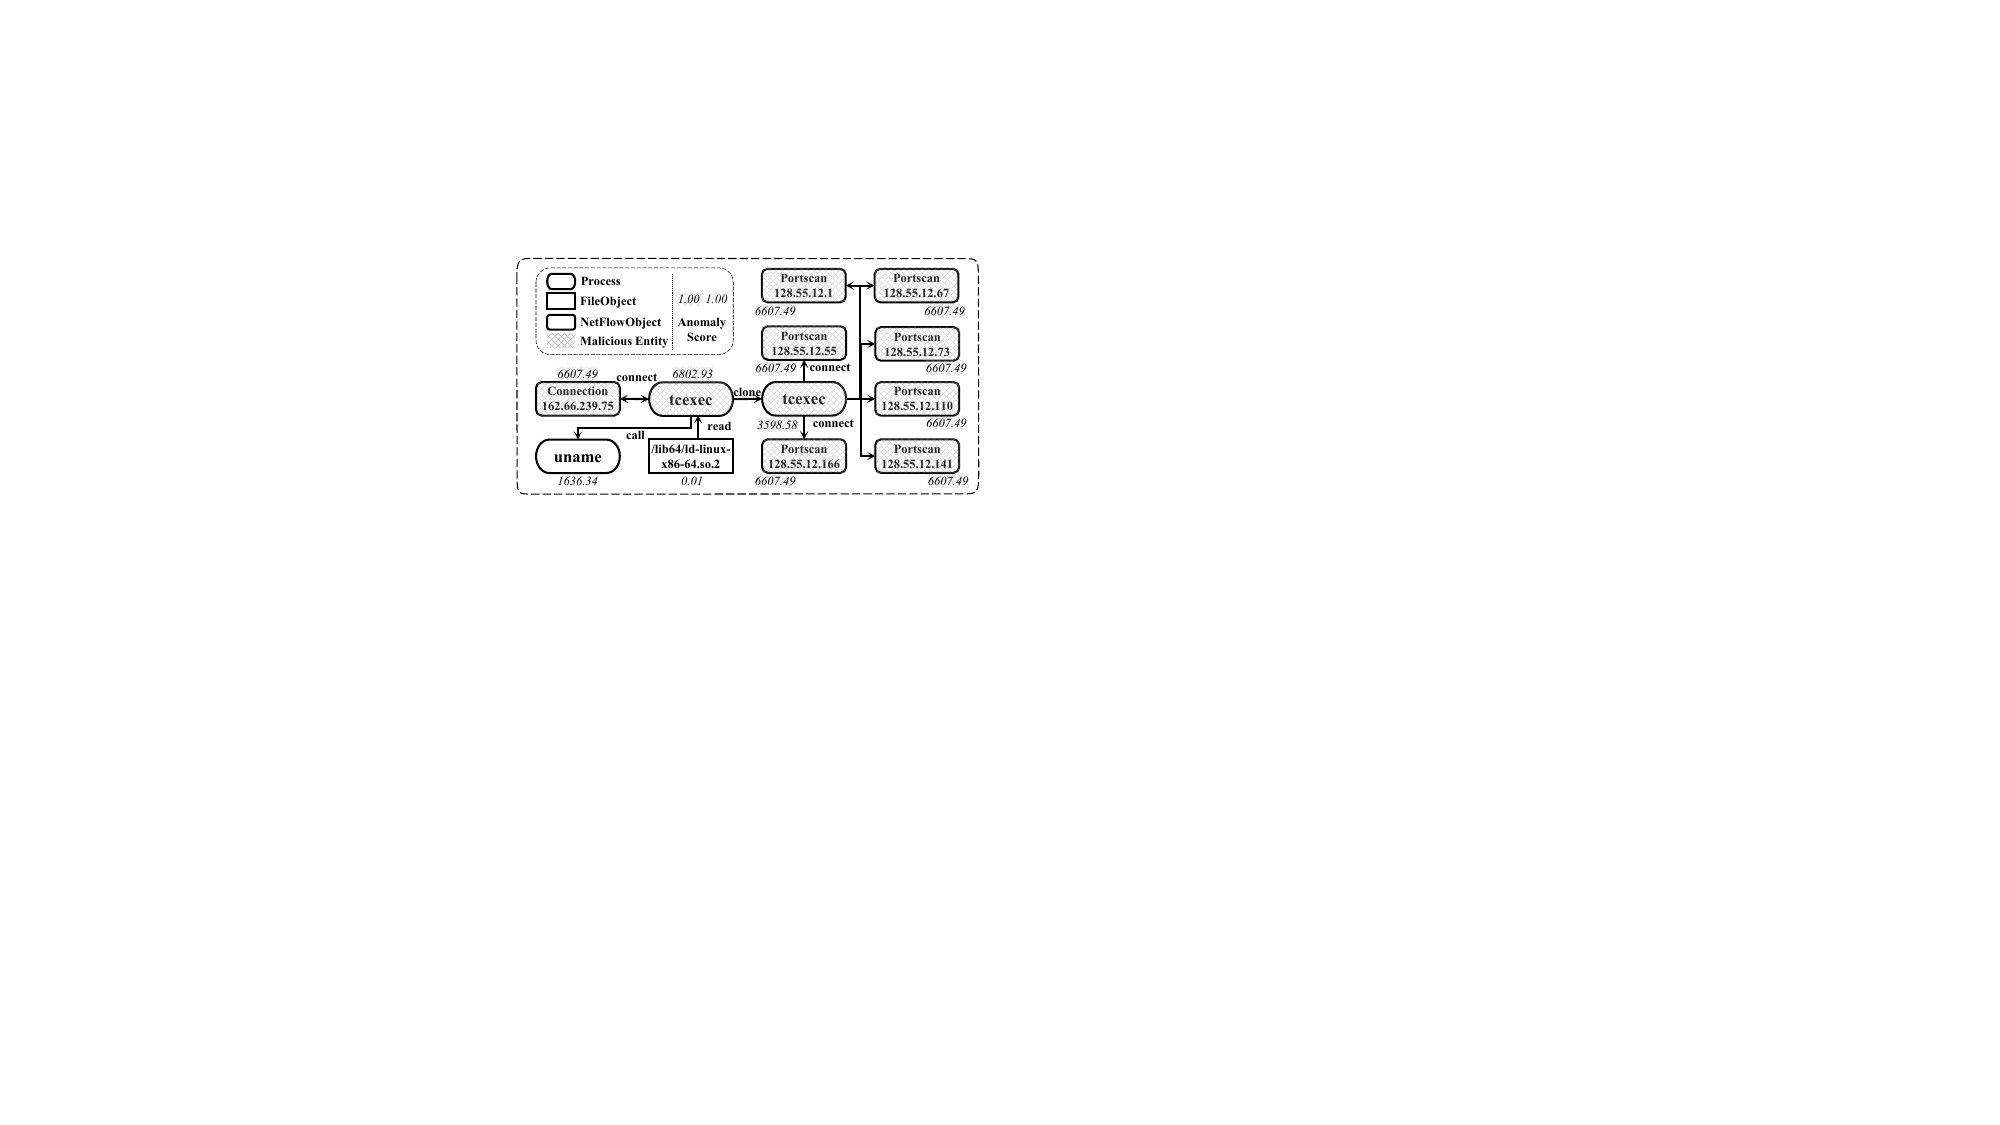}
    \caption{Another provenance graph of our motivating example (i.e. Pine Backdoor). Red nodes represent ground-truth malicious entities and black nodes are benign ones. Numbers assigned to nodes are their corresponding anomaly scores, assessed by \system{}'s detection module.}
    \label{fig_case_revised_letter}
\end{figure}
\section{Case Study}\label{sec_evaluation_6_revised}

We use our motivating example described in Sec.~\ref{sec_motivation_1_revised} again to illustrate how \system{} detect APTs from audit logs. Our motivating example involves an APT attack: Pine Backdoor, which implants an malicious executable to a host via phishing e-mail, aiming to perform internal reconnaissance and build a silent connection between the host and the attacker. We perform \emph{system entity level detection} on it and obtain real detection results from \system{}. First, \system{} constructs a provenance graph from raw audit logs. We present another example provenance graph in Figure~\ref{fig_case_revised} to illustrate, with some benign entities and interactions remain uncut this time. Among them, \emph{tcexec}, \emph{Connection-162.66.239.75} and the \emph{portscan} NetFlowObjects which \emph{tcexec} connects are malicious entities while the others are benign ones. The graph representation module then obtains their embeddings via the graphs masked auto-encoder. The embedding of \emph{tcexec} is calculated by propagating and aggregating information from its multi-hop neighborhood to model its interaction behavior with other system entities. For instance, its 2-hop neighborhood is namely \emph{Connection-162.66.239.75}, \emph{tcexec}'s sub-process, \emph{uname}, \emph{ld-linux-x86-64.so.2} and other portscan \emph{NetFlowObject}s. The detection module subsequently calculate distances between those embeddings and their k-nearest benign neighbors in the latent space and assigns anomaly scores to them. The malicious entities are given very high anomaly scores (3598.58\textasciitilde6802.93) that far exceed our detection threshold (3000) while others present low abnormality (0.01\textasciitilde1636.34). Thus, \system{} successfully detect malicious system entities with no false alarm generated.

\section{Implementation details}\label{appe_e_revised}

Our experiments are performed on a linux desktop computer with an Intel Core i7-12700K CPU, 32GB physical memory and a NVIDIA RTX 3090 GPU. For code-level implementation details, we developed several log parsers to cope with different format of audit logs, including a simple StreamSpot format~\cite{streamspot-35} and more complex ones such as Camflow~\cite{camflow-34}and CDM~\cite{cdm-36}. Provenance graphs are constructed using the graph processing library Networkx~\cite{networkx-37}. Those provenance graphs are generated and stored into an universal JSON format for the sake of compatibility. The graph representation module is implemented via PyTorch~\cite{pytorch-38} and the DGL library~\cite{dgl-40} and the detection module is developed with Scikit-learn~\cite{sklearn-39}. An Adam optimizer is used to optimize the graph representation module. In our hyper-parameter analysis, the dimension d of output embeddings is chosen from {16, 32, 64, 128, 256} , the number of GAT layers l in the graph encoder from {1, 2, 3, 4} and the mask rate of nodes from {0.3, 0.5, 0.7}. For the threshold $\theta$, it is chosen between 1 and 10 in batched log level detection. In entity level detection, $\theta$ is searched between 1000 and 6500.

\section{Response to Major Revision Requirements}

\subsection*{Letter to reviewers and shepherd}

Dear Reviewers and Shepherd,
\vspace{0.5em}

Thank you for your valuable comments
and suggestions! The following is a summary of our revision
actions to address the Major Revision Requirements, as well
as other comments in individual reviews. For your
convenience, we will repeat some of the new contents we
added to the paper – please pardon the redundancy.

In this response letter, all added/revised texts in the paper
are highlighted in blue. 
%Due to the tremendous changes we made to both our experiments and the paper, we first provide a summary of changes, and then address our revision following the revision requirements/comments order. 
For your review convenience we have also generated a PDF-diff version, attached after this letter.

Thanks again.
\vspace{0.5em}

\noindent Sincerely,
\vspace{0.5em}

\noindent Authors of Submission \#490

\subsection{Revision Summary}

Following the revision criteria (A2, A5) and the follow-up discussions in HotCRP, we have made the following changes:

\subsubsection{Evaluation}
\noindent\textit{Describe the labeling methodology used to label this (Trace) dataset and complete the missing statistics in Table 2.}

\begin{itemize}
    \item We have clarified that we use the same ground-truth labels on DARPA datasets as ThreaTrace ~\cite{aptlearnbasedthreatrace-17} (Sec.~\ref{sec_evaluation_1_revised}).
    \item Previously we uploaded a pdf document and discussed the labeling methodology used to obtain the ground-truth labels of the Trace dataset in A3. We have uploaded that document to our anonymous repository and we will make it public.
    \item We have updated Table 2 to include \#Node and \#Edge statistics. Since edges do not have labels, we do not report \#malicious edges (Sec.~\ref{sec_evaluation_1_revised}).
\end{itemize}

\noindent\textit{Apply this labeling methodology to StreamSpot and UnicornWget, then perform entity level detection on these datasets in addition to batched detection.}

\begin{itemize}
    \item In response A3, we clarified that due to lack of ground-truth, evaluating \system{}'s entity level detection on StreamSpot and Unicorn Wget datasets is impossible. We proposed to use DARPA THEIA and CADETS datasets instead, which was approved in response A5 by shepherd.
    \item Before carrying out experiments on DARPA THEIA and CADETS datasets, we have renewed our evaluation procedure of entity level detection on DARPA E3 datasets. We can now directly use the original batches of raw audit logs as input instead of splitting them into smaller batches before provenance graph construction. We report \system{}'s detection result and its performance overhead with a 80\% train ratio on the Trace dataset for comparison purpose. In corresponding to the above changes, we have updated all the experiments concerning \system{}'s entity level detection ability (Sec.~\ref{sec_evaluation_2_revised}). The updated experiments yield better results than previous experiments on the Trace dataset, thanks to improved code efficiency and the new experiment pipeline. 
    \item We have further evaluated \system{}'s entity level detection ability on DARPA E3 THEIA and CADETS datasets (Sec.~\ref{sec_evaluation_2_revised}).
\end{itemize}

\noindent\textit{Separate batched detection and entity detection in Figure 4 into multiple figures.}

\begin{itemize}
    \item We have separated batched detection and entity detection in the AUC Figure (Sec.~\ref{sec_evaluation_2_revised}).
    \item We have highlighted the level of detection in Table 3 (Sec.~\ref{sec_evaluation_2_revised}).
\end{itemize}

\noindent\textit{Separate results for the 4 TRACE attack scenarios reported in Table 2.}

\begin{itemize}
    \item We have provided more detailed detection results for the Trace dataset, concerning per-attack effectiveness (Sec.~\ref{sec_evaluation_2_revised}).
    \item We removed one of the attack scenario (i.e., \emph{Firefox Backdoor}), because among the four attack scenarios mentioned in the DARPA E3 ground truth document, the \emph{Firefox Backdoor} attack is a failed one and is not related to the other three attacks. ThreaTrace~\cite{aptlearnbasedthreatrace-17} also removed it from their experiments.
\end{itemize}

\noindent\textit{Clarify the AUC results -- The DARPA TRACE result looks like AUC=1, but Table 3 shows results are not perfect (~0.5\% FPR at the optimal point on the curve).}

\begin{itemize}
    \item We changed our evaluation metrics. Now we evaluate and report \system{}'s performance on \emph{Precision, Recall, False Positive Rate, F1-score} and \emph{AUC} (Sec.~\ref{sec_evaluation_2_revised}).
\end{itemize}

\subsubsection{Additional Experiments}

\noindent\textit{Add an evaluation of how the size of the log batches affect the results. The paper mentions that a batch with "250,000 edges is good enough," but "good enough" is not a sufficient justification. A solid evaluation of the trade-off between memory consumption and the effect of the batch size on accuracy is needed.}

\begin{itemize}
    \item Due to the changes in our experimental procedures described above, \system{} no longer need to split raw logs into smaller batches. Consequently, the concern over how would a changeable batch size impacts accuracy is no longer valid.
\end{itemize}

\noindent\textit{Choosing the batch size based on the number of edges may not be the right strategy; e.g., why not use time as guidance? Please evaluate the effect of the fixed edge-based batch size on time to detection (i.e., the delay between time of compromise and time of detection) and discuss/compare whether time-based sliding windows would perform worse/better.}

\begin{itemize}
    \item As explained earlier, this concern is no longer valid as well.
\end{itemize}

\subsubsection{Writing Changes and Clarifications}

\noindent\textit{It is not clear how the model would be used in a real-world setting in which the graph is dynamically updated. The response mentions using batches of logs. However, more details are needed in the paper to understand how this works in practice. Do you use overlapping sliding windows over the logs? If not, why not? Similarly, the paper should clarify missing details about its system such as a list of attributes MAGIC uses for each node and edge, and how the embedding vocabulary is constructed to handle dynamic changes (such as data that has new values for existing attributes).}

\begin{itemize}
    \item We have further explained \system{}'s detection pipeline, including what its individual components are supposed to do in training and inference phase, and a recommended two-stage detection approach (Sec.~\ref{sec_overview_revised}).
    \item We have re-written our explanation on \system{}'s graph construction steps to make it easier to understand (Sec.~\ref{sec_model_1_revised}).
\end{itemize}

\noindent\textit{Important technical details on how the model works, including how feature embeddings are derived in an inductive learning setting, how hyper-parameters are selected, and how the outlier detection thresholds are selected, are not clearly explained. Please provide additional information.}

\begin{itemize}
    \item We have explained how features and initial embeddings are obtained in our graph construction steps (Sec.~\ref{sec_model_1_revised}).
    \item We have clarified our hyper-parameter settings, including the fixed hyper-parameters and the grid search (Sec.~\ref{sec_implementation_revised} and Appendix~\ref{appe_e_revised}).
    \item We have expanded our ablation study (Sec.~\ref{sec_evaluation_5_revised}) to include an experiment regarding the detection threshold $\theta$ showing that $\theta$ is not sensitive. 
    \item We have provided a general guideline for hyper-parameter selection (Appendix~\ref{appe_f_revised}).
\end{itemize}

\noindent\textit{In general, the reviewers were in agreement that significant rewriting and improvements in paper presentation is needed to make the paper more accessible to a security audience. The paper needs to provide clear and intuitive definitions and concrete explanations for key components and processes of the system such as the nature of provenance graphs, the graph embedding process, and the denoising process.}

\begin{itemize}
    \item We have updated our text to clarify the definition of a provenance graph as well as our multi-granularity detection scheme (Sec.~\ref{sec_motivation_2_revised}).
    \item We have added explanation on the GAT layers in the graph representation module to provide a high-level overview on their functions (Sec.~\ref{sec_model_2_2_revised}).
    \item We have clarified the graph embedding process and the noise reduction process in our graph construction steps (Sec.~\ref{sec_model_1_revised}).
\end{itemize}

\subsubsection{Others}

Beyond the scope of the revision criteria mentioned in A2 and A5, we have made several new revisions, concerning the consistency of our paper and other constructive comments from multiple reviewers:

\begin{itemize}
    \item We have added an experiment regarding the impact of hyper-parameters on \system{}'s run-time overhead. And we have swapped the position of Sec. 6.5 Ablation Study and Sec. 6.4 Performance Overhead, so we can discuss \system{}'s efficiency first then talk about different factors affecting its efficiency later.
    \item We have discussed the possibility of adversarial attacks and added a simple experiment to evaluate \system{}'s robustness against log-manipulating adversaries (Sec.~\ref{sec_discussion_revised} and Appendix~\ref{appe_a_revised}).
    \item We have redone the false positive experiments with the new train ratio and reported a trackable positive rate (Sec.~\ref{sec_evaluation_3_revised}).
    \item We have re-checked our motivation example as well as the case study, concerning the correctness and intelligibility of both examples (Sec.~\ref{sec_motivation_1_revised} and Appendix~\ref{sec_evaluation_6_revised}).
    \item We have moved our case study to the appendix due to space constraints.
    \item We have revised all the figures included in our paper and ensured that they are readable in black and white.
    \item We have updated our code in the anonymous repository (\url{https://anonymous.4open.science/r/MAGIC-5787/}).
\end{itemize}

\subsection{Revision Details}

\vspace{0.5em}\noindent\textbf{MR1: Additional experiments on DARPA THEIA and CADETS datasets to further assess \system{}'s entity level detection ability. (Rev \#A).}\vspace{0.5em}

%We admit that one dataset (DARPA E3 Trace dataset) is not enough to demonstrate \system{}'s entity level detection power. 
As suggested, we have evaluated \system{} on three DARPA datasets: Trace, THEIA and CADETS. We have updated our experimental settings to catch up with this change: 

\textcolor{blue}{\noindent\textbf{DARPA E3 Datasets.} The DARPA Engagement 3 datasets (See Table~\ref{tab_entity_dataset_revised_letter}), as a part of the DARPA Transparent Computing Program, is collected among an enterprise network during an adversarial engagement.} and \textcolor{blue}{Trace, THEIA and CADETS sub-datasets are included in our evaluation. These three sub-datasets consist of a total 51.69GB of well-labeled records, containing as many as 6,539,677 system entities and 10,258,542 interactions. Thus, we evaluate \system{}'s \emph{system entity level detection} ability and address the overhead issue on these dataset.} 

\begin{table}[t]
\caption{Datasets for System Entity Level Detection.}
\label{tab_entity_dataset_revised_letter}
\resizebox{\columnwidth}{!}{
\begin{tabular}{|c|c|c|c|c|c|c|}
\hline
Dataset & Scenario & Malicious &\#Node &\#Edge & Size (GB)\\
\hline\hline
 \multirow{4}{*}{DARPA E3 Trace} & Benign & & 3,220,594 & \multirow{4}{*}{4,080,457} & \multirow{4}{*}{15.40}\\

 & Extension Backdoor & \checkmark & 732 & & \\

 & Pine Backdoor & \checkmark & 67,345 & & \\

 & Phishing Executable & \checkmark & 5 & & \\
 \hline\hline
 \multirow{2}{*}{DARPA E3 THEIA} & Benign & & 1,598,647 & \multirow{2}{*}{2,874,821} & \multirow{2}{*}{17.91}\\

 & Attack & \checkmark & 25,319 & & \\
\hline\hline
\multirow{2}{*}{DARPA E3 CADETS} & Benign & & 1,614,189 & \multirow{2}{*}{3,303,264} & \multirow{2}{*}{18.38}\\

 & Attack & \checkmark & 12,846 & & \\
\hline
\end{tabular}
}
\end{table}

And the evaluation results have also been re-aligned, including Table~\ref{tab_general_result_revised_letter}. \textcolor{blue}{On the DARPA datasets, \system{} achieves an average 99.91\% recall and 0.15\% false positive rate with only benign log entries for training. This indicates \system{} quickly learns to model system behaviors. The test set in this scenario is unbalanced, which means the total number of ground-truth benign entities far exceeds that of malicious entities. Specifically, only 106,246 of 1,386,046 test entities are labeled malicious.} 

\begin{table*}[t]
\caption{\system{}'s detection results on different datasets. For batched log level detection, the detection targets are log pieces. And for system entity level detection, system entities are the targets.}
\label{tab_general_result_revised_letter}
\resizebox{\linewidth}{!}{
\begin{tabular}{|c|c|c|c|c|c|c|c|c|c|c|c|c|c|c|}
\hline
\multirow{2}{*}{Granularity} & \multicolumn{2}{c|}{\multirow{2}{*}{Dataset}} & \multirow{2}{*}{Train Ratio} & \multicolumn{2}{c|}{Ground Truth} &\multirow{2}{*}{\#TP} &\multirow{2}{*}{\#FP} & \multirow{2}{*}{\#TN} & \multirow{2}{*}{\#FN} & \multirow{2}{*}{Precision} & \multirow{2}{*}{Recall} & \multirow{2}{*}{FPR} & \multirow{2}{*}{F1-Score} & \multirow{2}{*}{AUC}\\
\cline{5-6}

 & \multicolumn{2}{c|}{} & & \#Benign & \#Malicious & & & & & & & & &\\
\hline\hline
 
 \multirow{2}{*}{Batched log level} & \multicolumn{2}{c|}{StreamSpot} & 80\% & 100 & 100 & 100.0 & 0.59 & 99.41 & 0.0 & 99.41\% & 100.00\% & 0.59\% & 99.71\% & 99.95\%\\
 \cline{2-15}

 & \multicolumn{2}{c|}{Unicorn Wget} & 80\% & 25 & 25 & 24.0 & 0.5 & 24.5 & 1.0 & 98.02\% & 96.00\% & 2.00\% & 96.98\% & 96.32\%\\
 \hline\hline

 \multirow{6}{*}{System entity level} & \multirow{4}{*}{DARPA E3 Trace} & All & \multirow{4}{*}{80\%} & \multirow{4}{*}{616,025} & 68,082 & 68,072 & \multirow{4}{*}{569} & \multirow{4}{*}{615,456} & 10 & \multirow{4}{*}{99.17\%} & \multirow{4}{*}{99.98\%} & \multirow{4}{*}{0.09\%} & \multirow{4}{*}{99.57\%} & \multirow{4}{*}{99.99\%}\\
 \cline{3-3}\cline{6-7}\cline{10-10}

 & & Extension Backdoor & & & 732 & 727 & & & 5 & & & & &\\
 \cline{3-3}\cline{6-7}\cline{10-10}

 & & Pine Backdoor & & & 67,345 & 67,342 & & & 3 & & & & &\\
 \cline{3-3}\cline{6-7}\cline{10-10} 

 & & Phishing Executable & & & 5 & 3 & & & 2 & & & & &\\
 \cline{2-15}

 & DARPA E3 THEIA & All & 80\% & 319,448 & 25,319 & 25,318 & 456 & 318,992 & 1 & 98.23\% & 99.99\% & 0.14\% & 99.11\% & 99.87\%\\
 \cline{2-15}

 & DARPA E3 CADETS & All & 80\% & 344,327 & 12,846 & 12,816 & 759 & 343,568 & 30 & 94.40\% & 99.77\% & 0.22\% & 97.01\% & 99.77\%\\
 \hline

\end{tabular}}
\end{table*}

\vspace{0.5em}\noindent\textbf{MR2: Additional experiments on the impact of \system{}'s hyper-parameters on run-time overhead. (Rev \#B, C).}\vspace{0.5em}

We evaluated the impact of hyper-parameters in Sec.~\ref{sec_evaluation_5_revised}, including the embedding dimension $d$, number of GAT layers $l$ and mask rate $r$. Specifically, \textcolor{blue}{Figure~\ref{fig_hyperparameter_letter} illustrates how these hyper-parameters affect model performance in different situations. Hyper-parameters have little impact in most cases. Generally speaking, relatively higher model performance is achieved with a larger embedding dimension and more GAT layers by collecting more information from more distant neighborhoods, as shown in Sub-figure~\ref{fig_d_revised} and~\ref{fig_l_revised}. However, increasing $d$ or $l$ introduces heavier computation which leads to longer training and inference time.}

And, \textcolor{blue}{The default mask rate of $0.5$ yields best results. This is because \system{} is unable to get sufficient training under a low mask rate. And under a high mask rate, node features are severely damaged which prevents \system{} to learn node embeddings via feature reconstruction. Increasing mask rate slightly introduces more computation burden, as it increase the number of nodes involved in training the graph representation module.}

\begin{figure*}[t]
    \centering
    \setcounter{subfigure}{0}
    \subfigure[\textbf{\emph{d}}, on Wget dataset]{\includegraphics[width=0.330\hsize]{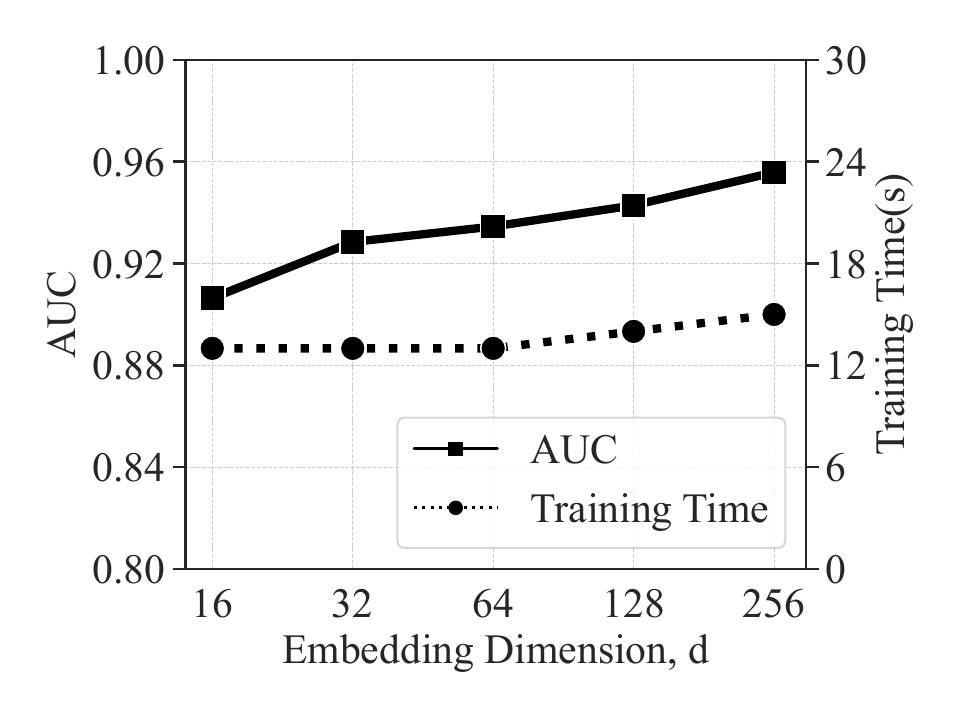}\label{fig_d_revised_letter}}
    \subfigure[\textbf{\emph{l}}, on Wget dataset]{\includegraphics[width=0.330\hsize]{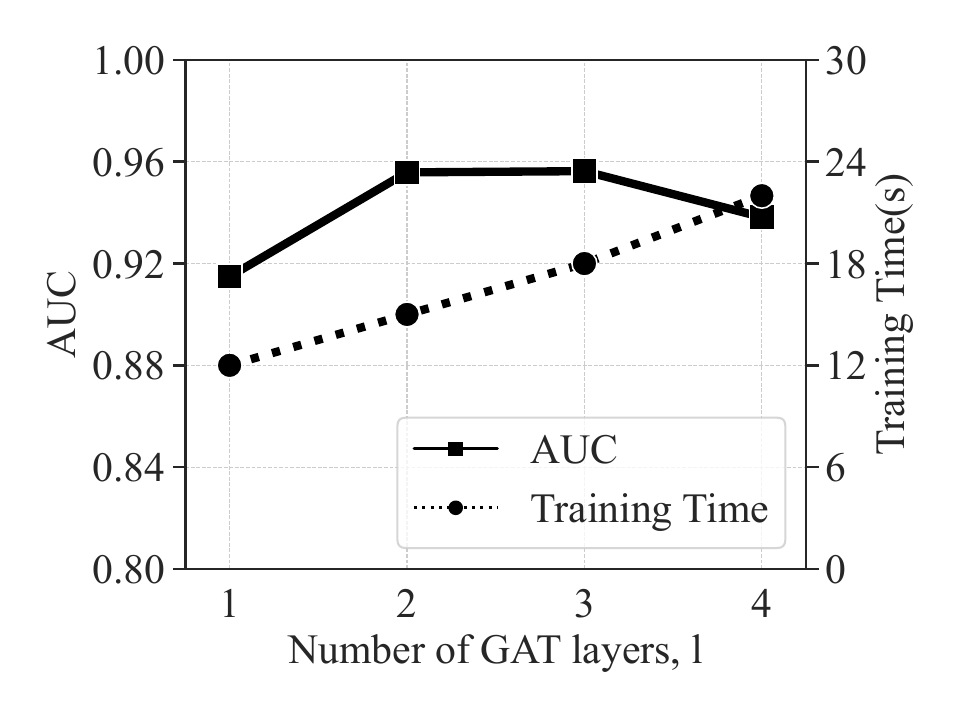}\label{fig_l_revised_letter}}
    \subfigure[\textbf{\emph{r}}, on Wget dataset]{\includegraphics[width=0.330\hsize]{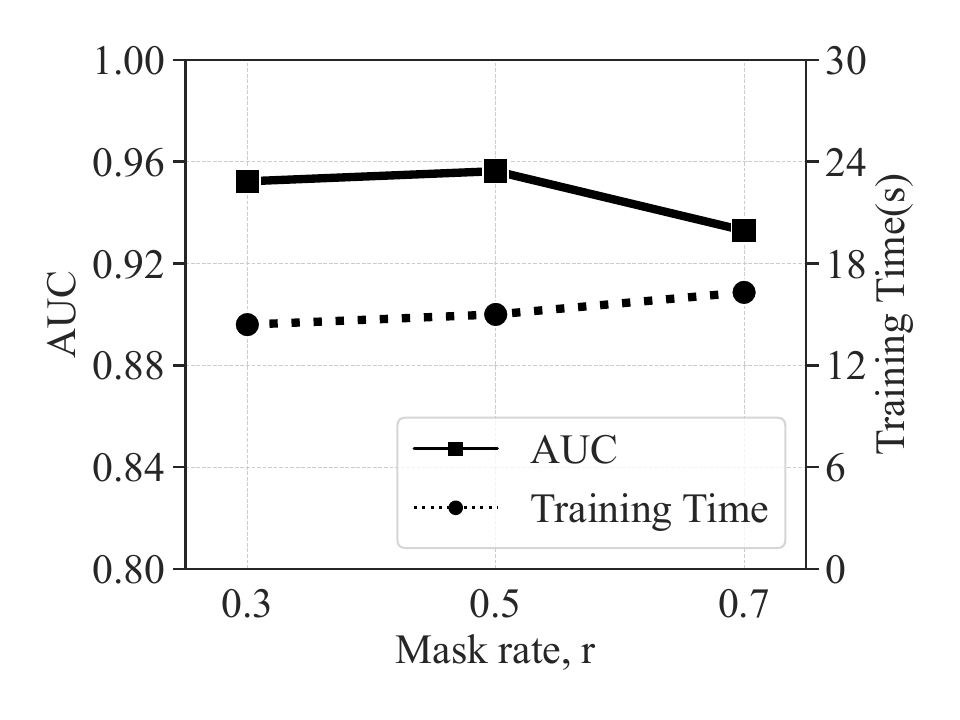}\label{fig_r_revised_letter}}
    \caption{Effect of different hyper-parameters on \system{}'s performance and efficiency.}
    \label{fig_hyperparameter_letter}
\end{figure*}
\vspace{0.5em}\noindent\textbf{MR3: Demonstrate \system{}'s robustness against adversarial attacks (Rev \#A, C).}\vspace{0.5em}

We have addressed this concern in two ways. First, we clarify in our threat model that \system{} is \textit{not} designed to deal with adversaries such as evasion attacks and poison attacks. 

\textcolor{blue}{\noindent\textbf{Threat Model.} We assume that APT attackers come from outside a system and target valuable information within the system. An attacker may perform sophisticated steps to achieve his goal but leave trackable evidence in system audit logs. The combination of the system hardware, operating system and system audit softwares is our trusted computing base. Poison attacks and evasion attacks are not considered in our threat model.}

Then, we discuss the possibility of adversarial attack strategies against \system{} in Sec.~\ref{sec_discussion_revised} (Discussion and Limitations). We provided a simple experiment showing that \system{} is robust enough against log-manipulating adversaries, which are typically effective against graph-based detectors.

\textcolor{blue}{
\noindent\textbf{Adversarial Attacks.} In Sec.~\ref{sec_evaluation_2_revised}, we show that \system{} handles stealth attacks well, which avoid detection by behaving similar to the benign system. However, if attackers get to know how \system{} work in details, they might conduct elaborately designed attacks to infiltrate our detector. We make a simple analysis on adversarial attacks and demonstrate \system{}'s robustness against them in Appendix~\ref{appe_a_revised}. As Graph-based approaches become increasingly popular and powerful in different detection applications, designing and avoiding these adversarial attacks on both the input graphs and the GNNs stands for an interesting research topic.}

In Appendix~\ref{appe_a_revised}, \textcolor{blue}{Adversarial attacks such as evasion attacks and poison attacks are tricky to implement but still possible to carry out. Two types of adversarial attacks are potentially practical against \system{}, manipulating input audit logs or exploiting model architecture. The later approach is not an option for \system{}'s attackers, as they have no access to \system{}'s inner parameters. Similar to SIGL~\cite{aptlearnbasedsigl-58}, we conduct a simple experiment concerning \system{}'s robustness against graph manipulations, which shows these attacks do not affect \system{}'s detection effectiveness. }

\textcolor{blue}{In this experiment, we expect attackers have no knowledge of \system{}'s inner parameters and cannot get any feedback from \system{}. However, attackers can freely manipulate the malicious entities within \system{}'s input audit logs, as well as a small proportion of benign entities. Consequently, we consider four types of attacks:}

\textcolor{blue}{\textbf{Malicious Feature Evasion (MFE).} Attackers have altered the features of all malicious entities in the raw audit logs trying to evade detection. This affects the node initial embeddings of the input provenance graph and forces malicious entities to mimic benign ones in node features.}

\textcolor{blue}{\textbf{Malicious Structure Evasion (MSE).} Attackers have adding new edges between malicious entities and benign ones, so that malicious entities behave more normally and tend to have local structures more similar to benign entities. This affects the graph representation module and pull the output embeddings of malicious nodes towards benign ones, making them more difficult to identify.}

\textcolor{blue}{\textbf{Combined Evasion (MCE).} This type of attack is a combination of the MFE and MSE and causes malicious entities to approximate benign ones in both features and structures.}

\textcolor{blue}{\textbf{Benign Feature Poison (BFP).} Attackers have manipulated the features of entities to poison \system{}. Attackers injected some benign entities with similar initial features as malicious entities, trying to convince \system{} that the malicious entities behave normally. This shifts benign entities to mimic malicious ones in node features, gradually poisons \system{}'s detection module.}

\textcolor{blue}{We evaluated \system{}'s robustness against the above four attack strategies on the Trace dataset and we present the results in Table~\ref{tab_adversarial}. Experimental results confirms that \system{} is robust enough against adversarial attacks. MFE has almost no impact on \system{}'s effectiveness. \system{} is slightly more vulnerable facing the structure evasion attacks, because the graph structure is critical to unsupervised graph representation learning. However, the structure attacks still have little impact on \system{}'s detection effectiveness. We believe that the feature and structure reconstruction involved in our graph representation module contributes to this robustness, as it learns a model to reconstruct both node features and its neighboring structure with the information from its neighbors. Consequently, adversarial attacks involving feature and structure altering of malicious entities will fail, and with \system{}'s model itself well-protected, attackers have to either extend their effort on searching and manipulating benign entities, or find other attack strategies against \system{}. Meanwhile, BFP has a relatively greater impact on \system{}'s performance. However, under BFP, only 0.057 AUC reduction is achieved by manipulating the input feature of an enormous 161,029 benign entities. This level of interference in the benign system is beyond the capability of ordinary attackers. Consequently, an effective BFP attack is also very difficult to carry out.}

\vspace{0.5em}\noindent\textbf{MR4: Clarify the nature of a provenance graph (Rev \#E).}\vspace{0.5em}

We apologize for the unclear explanations on our definitions, \system{}'s detection pipeline as well as the graph construction steps and the graph representation module. Here we clarify the definition of a provenance graph as \textcolor{blue}{\noindent\textbf{Provenance Graph.} A provenance graph is a directed cyclic graph extracted from raw audit logs. The construction of a provenance graph is common practice in data provenance, as it connects system entities and presents the interaction relationships between them. A provenance graph contains nodes representing different system entities (e.g., processes, files and sockets) and edges representing interactions between system entities (e.g., execute or connect), labeled with their types. For example, \emph{/tmp/tcexec} is a \emph{FileObject} system entity and the edge between \emph{/tmp/tcexec} and \emph{tcexec} is an \emph{execute} operation from a \emph{FileObject} targeting a \emph{Process}, as illustrated in Figure~\ref{fig_motivation_revised_letter}.}

\begin{figure}[t]
    \centering
    \includegraphics[width=0.495\textwidth]{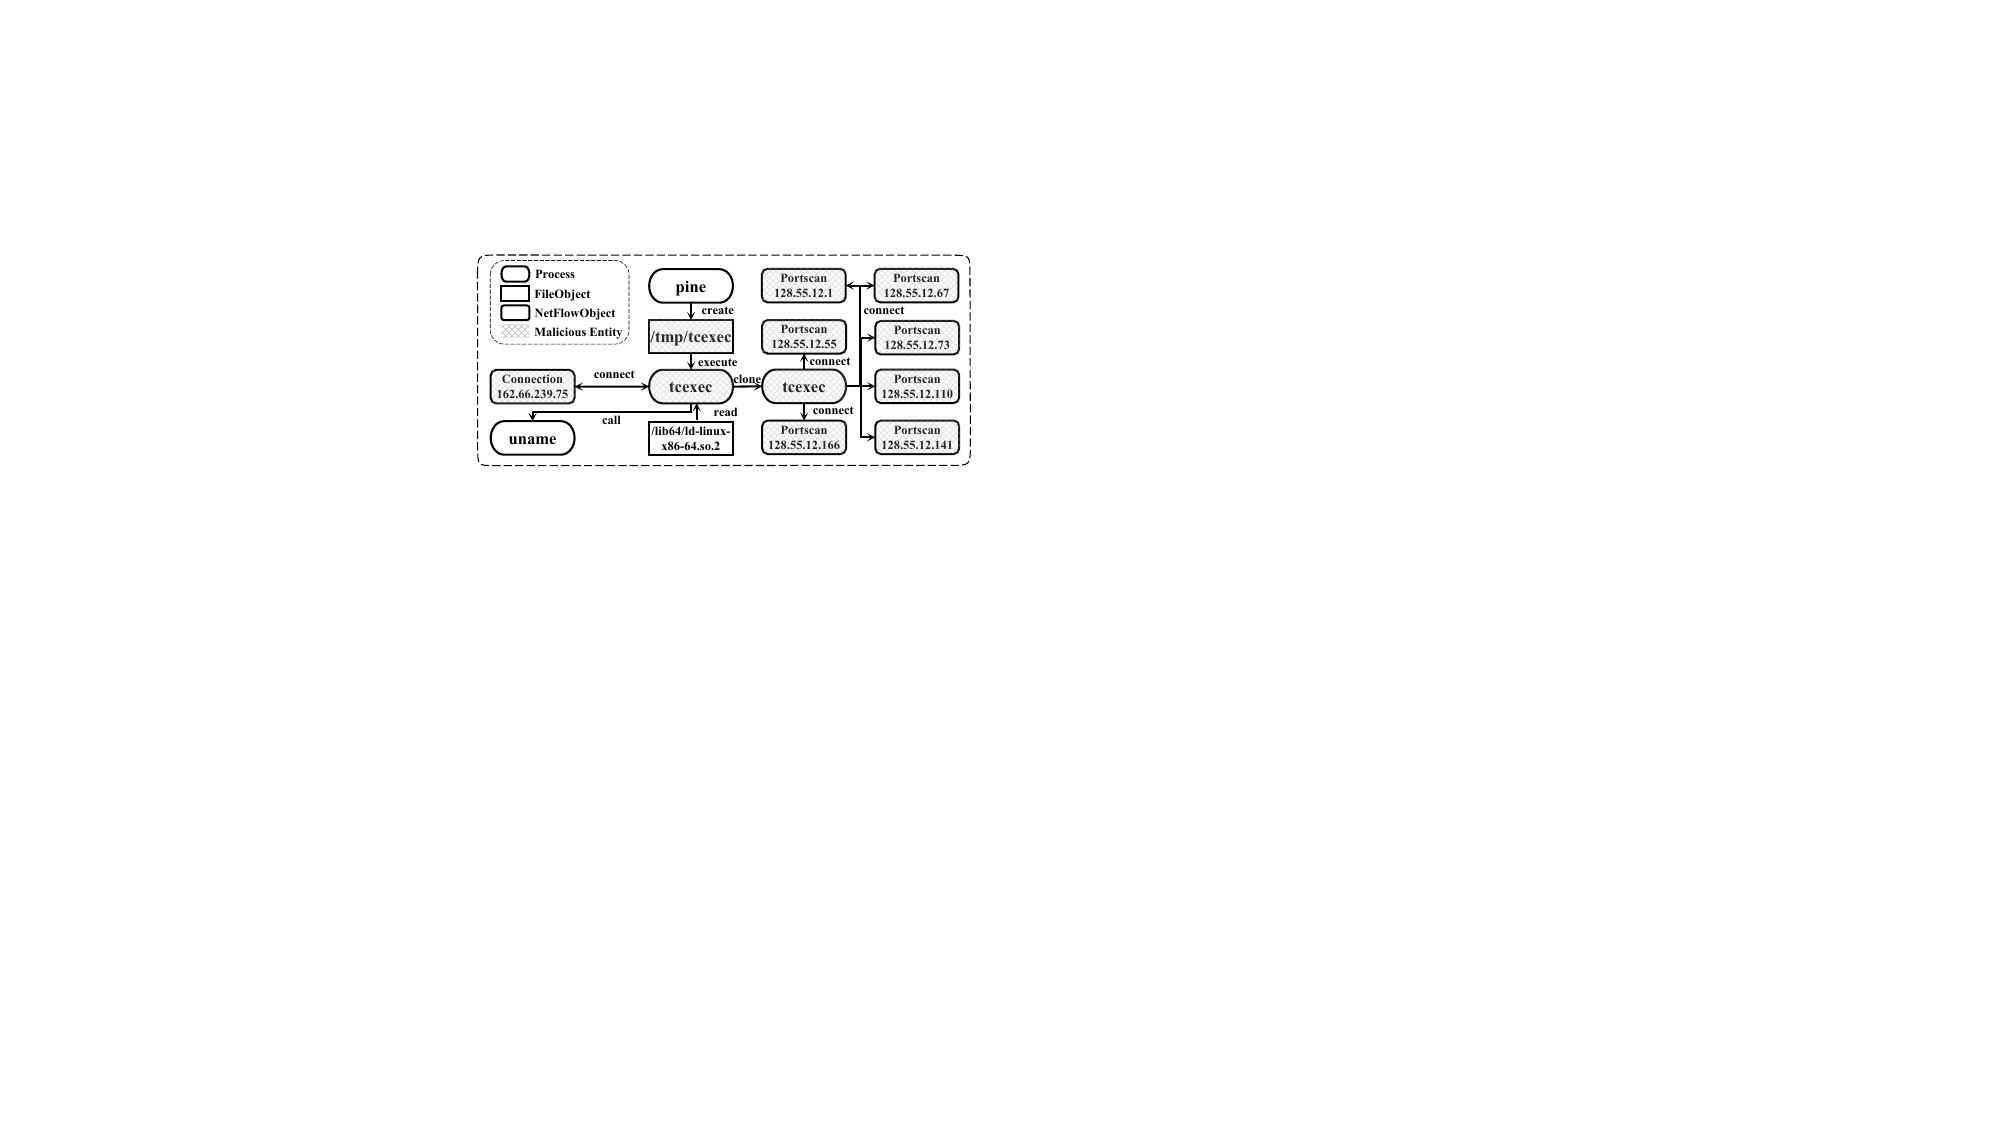}
    \caption{The provenance graph of a real-world APT attack, exploiting the Pine Backdoor vulnerability. All attack-irrelevant entities and interactions have been removed from the provenance graph.}
    \label{fig_motivation_revised_letter}
  \end{figure}
\vspace{0.5em}\noindent\textbf{MR5: Explain the fractions in the experimental results (Rev \#B).}\vspace{0.5em}

We have clarified in Sec.~\ref{sec_implementation_revised} (Implementation) that \textcolor{blue}{During evaluation, the average performance of \system{} under 100 global random seeds is reported as the final result, so the experimental results may contain fractions of system entities/batches of logs.}

\vspace{0.5em}\noindent\textbf{MR6: Clarify MAGIC's multi-granularity detection scheme and explain how it can be applied to real-world practice (Rev \#B).}\vspace{0.5em}

We have updated our description of \system{}'s multi-granularity detection ability in Sec.~\ref{sec_definition_revised} Threat Model and Definitions and also explained why such ability is needed and how it may work in real-world settings: \textcolor{blue}{\system{} is capable to perform APT detection at two-granularity: \emph{batched log level} and \emph{system entity level}. \system{}'s multi-granularity detection ability gives rises to a two-stage detection approach: first conduct batched log level detection on streaming batches of logs, and then perform system entity level detection on positive batches to identify detailed detection results. Applying this approach to real-world settings will effectively reduce workload, resource consumption and false positives and, in the meantime, produce detailed outcomes.}

\textcolor{blue}{\vspace{3pt}\noindent$\bullet$~ Batched log level detection. Under this granularity of APT detection, the major task is \emph{given batched audit logs from a consistent source, \system{} alerts if a potential APT is detected in a batch of logs}. Similar to Unicorn~\cite{aptlearnbased-10}, \system{} does not accurately locate malicious system entities and interactions under this granularity of detection.}

\textcolor{blue}{\vspace{3pt}\noindent$\bullet$~ System entity level detection. The detection task under this granularity of APT detection is \emph{given audit logs from a consistent source, \system{} is able to accurately locate malicious system entities in those audit logs}. Identification of key system entities during APTs is vital to subsequent tasks such as attack investigation and attack story recovery as it provides explicable detection results and reduces the need for domain experts as well as redundant manual efforts~\cite{aptlearnbasedatlas-11}.}

\vspace{0.5em}\noindent\textbf{MR7: Revise the sections concerning \system{}'s overview and clarify \system{}'s detection pipeline (Rev \#B, D, E).}\vspace{0.5em}

We failed to make things clear in our previous version of paper and here we provide some background of \system{}'s detection pipeline. \system{} takes as input the raw audit logs recorded and stored by system auditing softwares (or devices). These softwares (or devices) yields audit logs \emph{in batches}, which means the raw input of \system{}'s detection pipeline is static batches of logs. We do not fuse these batches into one to preserve the scalability of \system{}. \system{}'s graph construction steps need to be performed on every log batches, resulting in one provenance graph for each batch. 

During training, \system{} first transform training log batches in to training provenance graphs through graph construction steps, then the graph representation module is trained upon these training graphs and updates its inner parameters. The graph representation module also compute output embeddings (system state embeddings for batched log level and node embeddings for system entity level) of these graphs for the detection module, as the training embeddings. The detection module takes these embeddings as training samples and memorize them.

During inference, the test log batches also need to be transformed into test provenance graphs, through \system{}'s graph construction steps. The graph representation module, in its inference mode, simply computes output embeddings from the test graphs and feed them to the detection module, as the target embeddings. The detection module then perform outlier detection on target embeddings, with the memorized training embeddings as the ground-truth distribution.

\begin{figure*}[t]
    \centering
    \includegraphics[width=0.99\hsize]{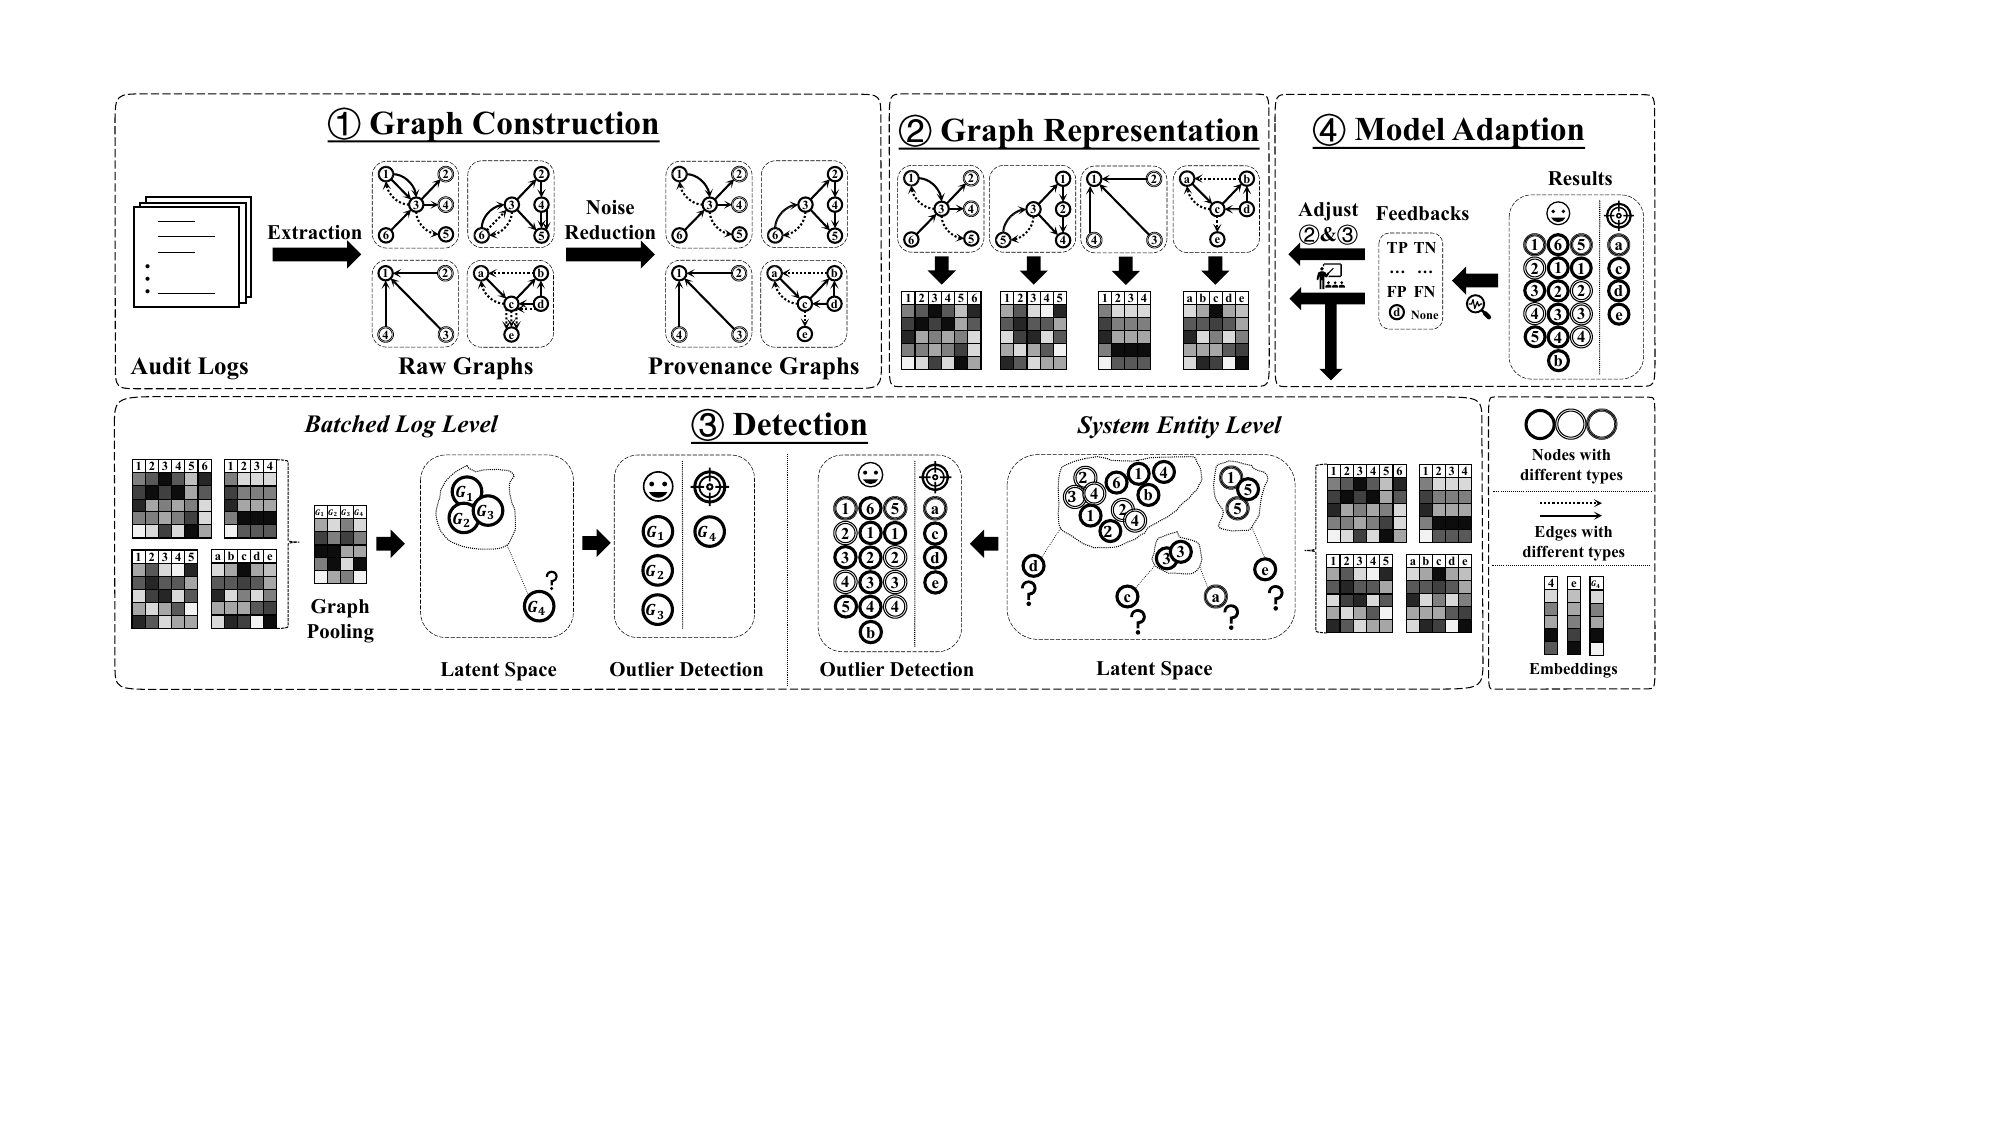}
    \caption{Overview of \system{}'s detection pipeline.}
    \label{fig_overview_revised_letter}
  \end{figure*}
\textcolor{blue}{system{} is a novel self-supervised APT detection approach that leverages masked graph representation learning and outlier detection methods and is capable of efficiently performing multi-granularity detection on massive audit logs. \system{} consists of three main steps: (1) constructing a provenance graph, (2) learning a graph representation module and (3) performing outlier detection. It also provides an optional (4) model adaption mechanism. Figure~\ref{fig_overview_revised_letter} gives an overview of the \system{} architecture.}

\textcolor{blue}{Streaming audit logs collected by system auditing softwares are stored in batches in common practice. During provenance graph construction (1), \system{} transforms these logs into static provenance graphs. System entities and interactions between them are extracted and converted into nodes and edges respectively. Several complexity reduction techniques are utilized to remove redundant information.
}

\textcolor{blue}{The constructed provenance graphs are then fed through the graph representation module (2) to obtain embeddings (i.e. comprehensive vector representations of objects). Built upon \emph{graph masked auto-encoders} and integrates \emph{sample-based structure reconstruction}, the graph representation module embeds, propagates and aggregates node and edge attributes into output embeddings, which contain both node embeddings and the system state embedding.}

\textcolor{blue}{The graph representation module is trained with only benign audit logs to model benign system behaviors. When performing APT detection on potentially attack-containing audit logs, \system{} utilizes \emph{outlier detection methods} based on the output embeddings to detect outliers in system behaviors (3). Depending on the granularity of the task, different embeddings are used to complete APT detection. When performing \emph{batched log level detection}, the system state embeddings, which reflect the general behaviors of the whole system, are the targets of outlier detection. An outlier in such embeddings means its corresponding system state is unseen and potentially malicious, which reveals an APT signal in that batch of audit logs. When performing \emph{system entity level detection}, the detection targets are those node embeddings, which represent the behaviors of system entities. Outliers in node embeddings, however, indicates suspicious system entities and detects APT threats in finer granularity.}

\textcolor{blue}{In real-world detection settings, \system{} has two pre-designed applications.  For each batch of logs collected by system auditing softwares, one can either directly utilize \system{}'s entity level detection to accurately identify malicious entities within the batch, or perform a two-stage detection, as stated in~\ref{sec_definition_revised}. In this case, \system{} first scans the batch and sees if malicious signals exist in a batch (batched log level detection). If it alerts positive, \system{} then performs entity level detection to identify malicious system entities in finer granularity. Batched log level detection is significantly less computationally demanding than entity level detection. Therefore, such a two-stage routine can help \system{}'s users to save computational resource and avoid false alarms without affecting \system{}'s detection fineness. However, if users favor fine-grain detection on all system entities, the former routine is still an accessible option.}

\textcolor{blue}{To deal with \emph{concept drift}, potential stealth attacks and unseen attacks, an optional model adaption mechanism is employed to provide feedback channels for its users (4). Detection results checked and confirmed by security analysts are fed back to \system{}, helping it to adapt to benign system behavior changes in a semi-supervised way. Under such semi-supervised conditions, \system{} achieves even more promising detection results, which is discussed in Sec.~\ref{sec_evaluation_5_revised}. Furthermore, \system{} can be easily applied to real-world online APT detection thanks to it's ability to adapt itself to \emph{concept drift} and its minimum computation overhead.}

\vspace{0.5em}\noindent\textbf{MR8: Clarify \system{}'s graph construction steps and the embedding layer (Rev \#B, D, E).}\vspace{0.5em}

In short, \system{}'s pre-processing steps, including \system{}'s graph construction steps and the initial embeddings is doing the following things:

\begin{itemize}
    \item Generate one-column categorical features (i.e. types) for entities and interactions in the raw logs, which may have complex multi-column categorical features.
    \item Construct a multi graph from these entities and interactions, with entities as nodes and interactions as edges.
    \item Remove \emph{redundant} edges between node pairs. \emph{Redundant} edges refer to those edges with the same source and destination points as well as the same edge types. 
    \item Transform nodes and edges' types into one-hot initial embeddings.
    \item Between all node pairs, combine edges with different types into one by averaging the initial embeddings of these edges. Now the graph becomes a simple graph, where only one edge exists between a pair of source and destination nodes.
\end{itemize}

We have formalized the above steps in the revised Sec.~\ref{sec_model_1_revised} Provenance Graph Construction. Previously, we put our explanation on initial embeddings in Sec. 4.2.1. Now, we moved it to Sec.~\ref{sec_model_1_revised} Provenance Graph Construction and we focus on the feature masking in Sec.~\ref{sec_model_2_1_revised}. We have also provided a visual example of the graph construction steps to support the descriptive text.

Another clarification we have made is concerning the universe of initial embeddings. The dimension of node/edges' initial embeddings, noted by $t$, equals to the number of possible node/edge types. This number is determined by the input data format and is fixed if the system auditing software (or device) is not replaced by a new one. Thus, our initial embedding scheme works under a transductive setting and there is no unseen labels (types).

\textcolor{blue}{\system{} first constructs a provenance graph out of raw audit logs before performing graph representation and APT detection. We follow three steps to construct a consistent and optimised provenance graph ready for graph representation.}

\textcolor{blue}{\noindent\textbf{Log Parsing.} The first step is to simply parse each log entry, extract system entities and system interactions between them. Then, a prototype provenance graph can be constructed with system entities as nodes and interactions as edges. Now we extract categorical information regarding nodes and edges. For simple log format that provides entity and interaction labels, we directly utilize these labels. For some format that provides complicated attributes of those entities and interactions, we apply multi-label hashing (e.g., xxhash~\cite{xxhash-27}) to transform attributes into labels. At this stage, the provenance graph is a directed multi-graph. We designed an example to demonstrate how we deal with the raw provenance graph after log parsing in Figure~\ref{fig_gc_revised_letter}.}

\textcolor{blue}{\noindent\textbf{Initial Embedding.} In this stage, we transform node and edge labels into fixed-size feature vector (i.e., initial embedding) of dimension $d$, where $d$ is the hidden dimension of our graph representation module. We apply a \emph{lookup embedding}, which establish an one-to-one mapping between node/edge labels to $d$-dimension feature vectors. As demonstrated in Figure~\ref{fig_gc_revised} (I and II), process \emph{a} and \emph{b} shares the same label, so they are mapped to the same feature vector, while \emph{a} and \emph{c} are embedded into different feature vector as they have different labels. We note that the possible number of unique node/edge labels is determined by the data source (i.e., auditing log format). Therefore, the lookup embedding works under a transductive setting and do not need to learn embeddings for unseen labels.}

\begin{figure}[t]
    \centering
    \includegraphics[width=0.495\textwidth]{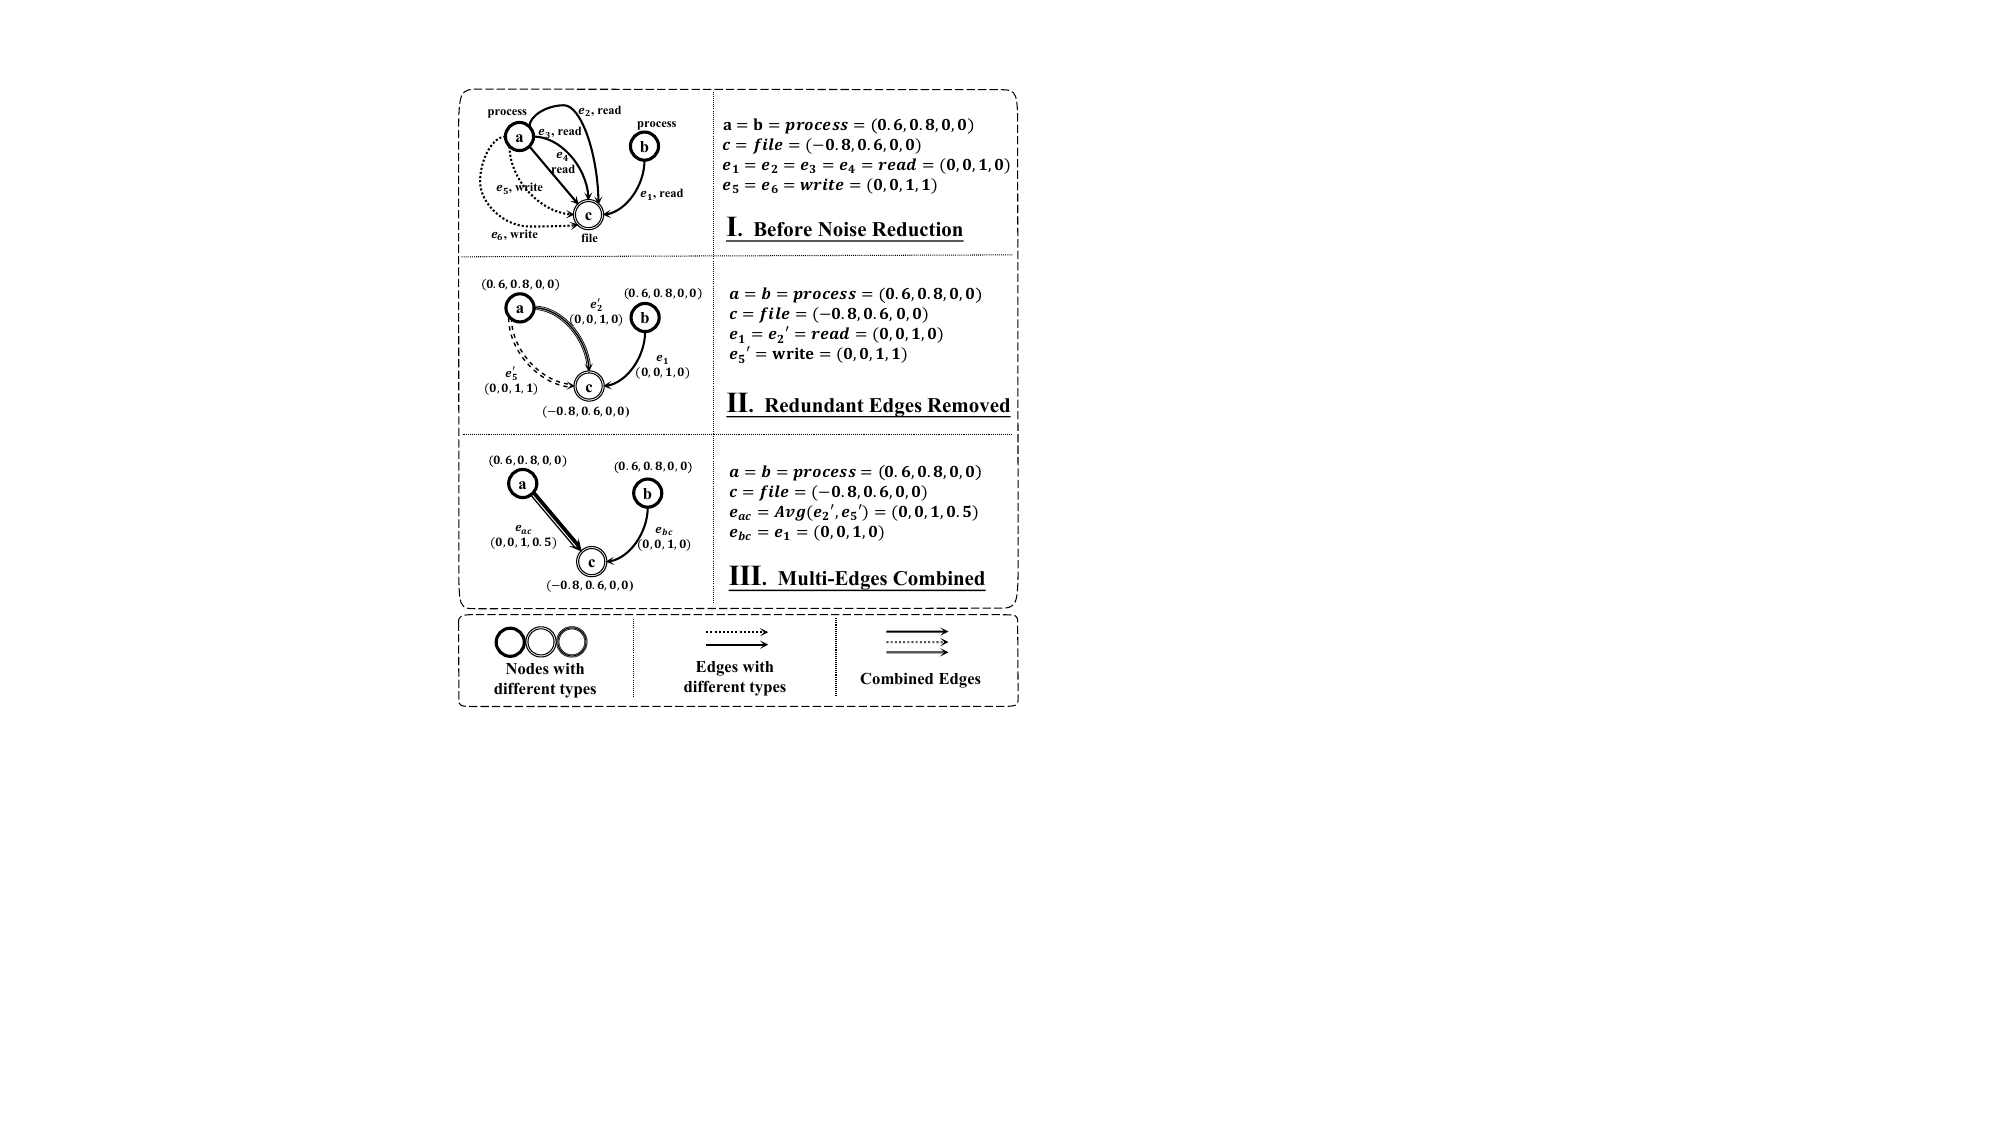}
    \caption{Example of \system{}'s graph construction steps.}
    \label{fig_gc_revised_letter}
  \end{figure}
\textcolor{blue}{\noindent\textbf{Noise Reduction.} The expected input provenance graph of our graph representation module would be simple-graphs. Thus, we need to combine multiple edges between node pairs. If multiple edges of the same label (also sharing the same initial embedding) exist between a pair of nodes, we remove redundant edges so that only one of them remains. Then we combine the remaining edges into one final edge. We note that between a pair of nodes, edges of several different labels may remain. After the combination, the initial embedding of the resulting unique edge is obtained by averaging the initial embeddings of the remaining edge. To illustrate, we show how our noise reduction combine multi-edges and how it affects the edge initial embeddings in Figure~\ref{fig_gc_revised} (II and III). First, three \emph{read} and two \emph{write} interactions between \emph{a} and \emph{c} are merged into one for each label. Then we combine them together, forming one edge $e_{ac}$ with initial embedding equal to the average initial embedding of the remaining edges ($e_2^{\prime}$ and $e_5^{\prime}$). We provide a comparison between our noise reduction steps and previous works in Appendix~\ref{appe_c_revised}.}

\textcolor{blue}{After conducting the above three steps, \system{} has finished constructing a consistent and information-preserving provenance graph ready for subsequent tasks. During provenance graph construction, little information is lost as \system{} only damages the original semantics by generalizing detailed descriptions of system entities and interactions into labels. However, an average 79.60\% of all edges are reduced on the DARPA E3 Trace dataset, saving \system{}'s training time and memory consumption.}

\vspace{0.5em}\noindent\textbf{MR9: Clarify \system{}'s graph encoder and the function of GATs (Rev \#B, E).}\vspace{0.5em}

Due to the changes described above, we have first re-established our description of \system{}'s feature masking: \textcolor{blue}{Before training our graph representation module, we perform \emph{masking} on nodes, so that the graph masked auto-encoder can be trained upon reconstruction of these nodes. Masked nodes are randomly chosen, covering a certain proportion of all nodes. The initial embeddings of such masked nodes are replaced with a special mask token $x_{mask}$ to cover any original information about these nodes. Edges, however, are not masked because these edges provide precious information about relationships between system entities. In summary, given node initial embedding $x_n$, we mask nodes as follows:
$$
\begin{aligned}
\begin{split}
emb_{n} &= 
\begin{array}{ll}
x_n, & {n \notin \widetilde{N}}\\
x_{mask}, & {n \in \widetilde{N}}
\end{array}
\end{split}
\end{aligned}
$$
where $\widetilde{N}$ are randomly-chosen masked nodes, $emb_n$ is the embedding of node n ready for training the graph representation module. This masking process only happens during training. During detection, we do not mask any nodes.}

In addition, we have altered our explanation on GAT layers to make sure that our readers fully understand them. \textcolor{blue}{The encoder of our graph representation module contains multiple stacked layers of graph attention networks (GAT)~\cite{gat-29}. The function of a GAT layer is to generate output node embeddings according to both the features (initial embeddings) of the node itself and its neighbors. Differing from ordinary GNNs, GAT introduces an attention mechanism to measure how important those neighbors are.}

\textcolor{blue}{To explain in detail, one layer of GAT takes node embeddings generated by previous layers as input and propagates embeddings from source nodes to destination nodes into messages along the interactions. The message contains information about the sources node and the interaction between source and destination:
$$
MSG(src, dst) = W_{msg}^T(h_{src}||emb_e).\\
$$}

\textcolor{blue}{And the attention mechanism is employed to calculate the attention coefficients between the message sources and their destinations:
$$
\begin{aligned}
\alpha(src, dst) &= LeakyReLU(W_{as}^Th_{src}+W_{am}MSG(src, dst)),\\
a(src, dst) &= Softmax(\alpha(src, dst)).\\
\end{aligned}
$$}

\textcolor{blue}{Then for the destination nodes, the GAT aggregates messages from incoming edges to update their node embeddings by computing a weighted sum of all incoming messages, whose weights are exactly the attention coefficients:
$$
\begin{aligned}
AGG(h_{dst}, h_{\mathcal{N}}) &= W_{self}h_{dst} + \sum_{i\in \mathcal{N}}a(i, dst)MSG(i, dst),\\
h_n^l &= AGG^l(h_n^{l-1}, h_{\mathcal{N}_n}^{l-1}).
\end{aligned}
$$
where $h_n^l$ is the hidden embedding of node $n$ at $l$-th layer of GAT, $h_n^{l-1}$ is that of layer $l-1$ and $\mathcal{N}_n$ is the one-hop neighborhood of $n$. The input of the first GAT layer is the initial node embedding. $emb_e$ is the initial edge embedding and remains constant throughout the graph representation module. $W_{as},W_{am},W_{self},W_{msg}$ are trainable parameters. The updated node embedding forms a general abstraction of the node's one-hop interaction behavior.}

\textcolor{blue}{Multiple layers of such GATs are stacked to obtain the final node embeddings $h$, which is concatenated by the original node embedding and outputs of all GAT layers:
$$
\begin{aligned}
h_n = emb_n || h_n^1 || \cdots || h_n^l.
\end{aligned}
$$
where $\cdot||\cdot$ denotes the concatenate operation. The more layers of GAT stacked, the wider the neighboring range is and the farther a node's multi-hop interaction pattern its embedding is able to represent. Consequently, the graph encoder effectively incorporates node initial features and multi-hop interaction behaviors to abstract system entity behaviors into node embeddings. The graph encoder also applies an average pooling to all node embeddings to generate a comprehensive embedding of the graph itself~\cite{graphpooling-30}, which recapitulates the overall state of the system:
$$
h_G = \frac{1}{|N|}\sum_{n_i\in N}h_{n_i}.
$$
The node embeddings and system state embeddings generated by the graph encoder are considered the output of the graph representation module, which are used in subsequent tasks in different scenarios.}

\vspace{0.5em}\noindent\textbf{MR10: Clarify the input of \system{}'s detection module, which is referred as \emph{graph embeddings} in previous versions (Rev \#B).}\vspace{0.5em}

We clarify here that the output of the graph representation layer are called \emph{output embeddings}, which contains both \emph{node embeddings} and \emph{system state embeddings}. The system state embedding is the result of graph pooling on all the node embeddings in a single graph. Consequently, a graph fed into the graph representation module may yields hundreds of nodes embeddings depending on the total number of nodes in the graph, but only one system state embedding. The input of the detection module depends on the detection granularity. Node embeddings for entity level detection and system state embeddings for batched log level detection. Specifically, \textcolor{blue}{The node embeddings and system state embeddings generated by the graph encoder are considered the output of the graph representation module, which are used in subsequent tasks in different scenarios.} Also, we have revised the whole paper to switch to these newly-defined terms.

\vspace{0.5em}\noindent\textbf{MR11: Explain in details the grid search conducted in \system{}'s experiments (Rev \#B, C).}\vspace{0.5em}

Default values of hyper-parameter $d$, $l$ and $r$ are used in most our experiments (except in the hyper-parameter analysis). We perform the search on the detection threshold $\theta$ separately on different datasets. On Unicorn Wget dataset, which contains specially designed stealthy attacks far from real-world APTs, we use half the test set for $\theta$ selection and the rest for testing. On other datasets, we use no more than 10\% of the test set for $\theta$ selection. We have updated Sec.~\ref{sec_implementation_revised} to provide more details on hyper-parameter settings: \textcolor{blue}{For hyper-parameters of MAGIC, the scaling factor $\gamma$ in the feature reconstruction loss is set to 3, the number of neighbors k is set to 10, the learning rate is set to 0.001 and the weight decay factor equals $5\times10^{-4}$. We use a 3 layer graph encoder and a mask rate of 0.5 in our experiments. The output embedding dimension d is different on two detection scenarios, batched log level detection and entity level detection. We use d equals 256 in batched log level detection and of and an we set d equals 64 in entity level detection to reduce resource consumption. The detection threshold $\theta$ is chosen by a simple linear search separately conducted on each dataset. The hyper-parameters may have other choices. We demonstrate the impact of these hyper-parameters on MAGIC later in the evaluation section. For other implementation details, we present them in Appendix~\ref{appe_e_revised}.}

And in Appendix~\ref{appe_e_revised}: \textcolor{blue}{ In our hyper-parameter analysis, the dimension d of output embeddings is chosen from {16, 32, 64, 128, 256} , the number of GAT layers l in the graph encoder from {1, 2, 3, 4} and the mask rate of nodes from {0.3, 0.5, 0.7}. For the threshold $\theta$, it is chosen between 1 and 10 in batched log level detection. In entity level detection, $\theta$ is searched between 1000 and 6500.}

In practice, even without attack data available, such a grid search is definitely not necessary. The hyper-parameter analysis in Sec.~\ref{sec_evaluation_5_revised} clearly indicates the impact of these parameters and we also provided a general guideline for hyper-parameter selection in Appendix~\ref{appe_f_revised}: \textcolor{blue}{or most hyper-parameters involved in \system{}, including $l$ and $r$, default choices works fine in all conditions. \system{}'s users may just select $l$ equals 2 or 3 and $r$ equals 0.5 in all applications. For the embedding dimension $d$, the choice is up to the user himself, as a higher $d$ results in better performance at the cost of resource consumption. The choice of detection threshold $\theta$ depends on the corresponding dataset \system{} is operating on. However, $\theta$ is not sensitive on individual datasets. Even if there is only benign data available, users may adjust and choose the optimal $\theta$ according to the resulting false positive rate (i.e. use the first $\theta$ when false positive rate is below the desired value).}

\vspace{0.5em}\noindent\textbf{MR12: The detection threshold $\theta$ is worrisome and the paper should demonstrate that $\theta$ is not sensitive in better ways or explain how to select an optimal $\theta$ (Rev \#B, D).}\vspace{0.5em}

Previously we failed to clearly explain why and how $\theta$ is not sensitive in proper ways. We have revised the hyper-parameter analysis in Sec.~\ref{sec_evaluation_5_revised} to better demonstrate this claim. Specifically, \textcolor{blue}{We further measured the anomaly score of embeddings in all datasets, which is demonstrated in Figure~\ref{fig_score_revised_letter}. A lower $\theta$ theoretically generates more false positives, as some unfamiliar system behaviors with relatively high anomaly scores are detected as outliers. Apparently, malicious embeddings are given extremely high anomaly scores compared with benign ones and they are well-separated from benign embeddings without overlapping. This support the claim that $\theta$ is not sensitive in practical situations and \system{} do not depends on a precise threshold $\theta$ to perform accurate APT detection. }

\begin{figure}[t]
    \centering
    \includegraphics[width=0.4\textwidth]{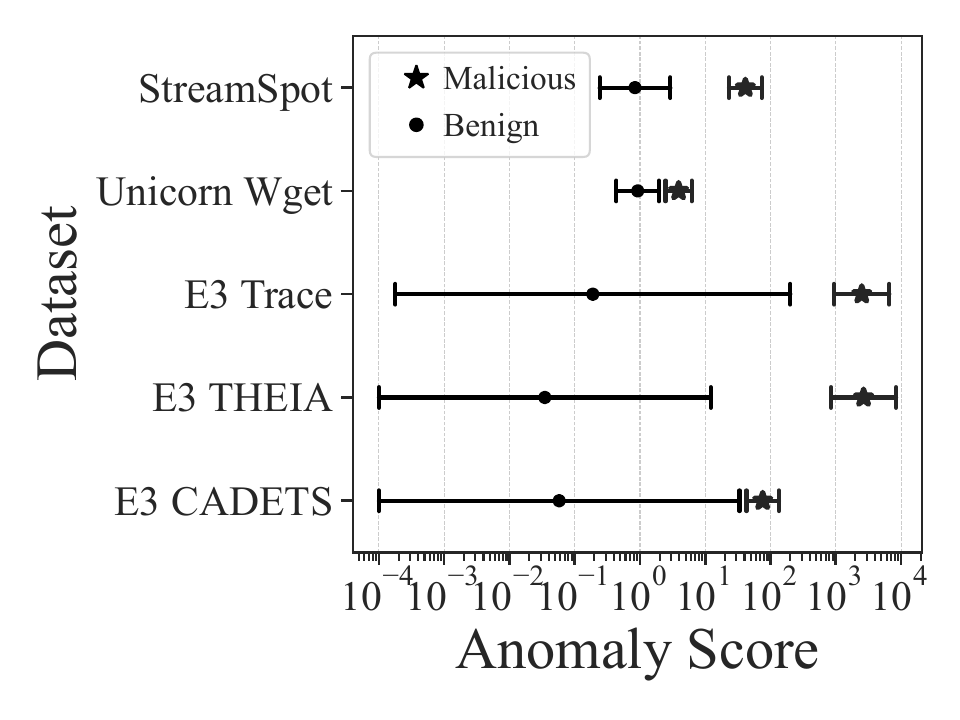}
    \caption{Distribution of anomaly scores of both benign and malicious entities, tested on all datasets.}
    \label{fig_score_revised_letter}
\end{figure}
Meanwhile, as stated earlier in \textbf{MR11}, we have provided a general guideline for hyper-parameter selection, including the threshold $\theta$.

\vspace{0.5em}\noindent\textbf{MR13: Provide a trackable false positive rate of \system{} (Rev \#C).}\vspace{0.5em}

We have demonstrated the number of total false alarms and the average number of false alarms each day in Sec.~\ref{sec_evaluation_3_revised} False Positive Analysis: \textcolor{blue}{\system{} yields low FPR (average 0.15\%) with large training data. This is because \system{} models benign system behaviors with self-supervised embeddings, allowing it to effectively handle unseen system entities. Such a low FPR enables \system{}'s application under real-world settings. When conducting fine-grain entity-level detection only, \system{} only yields 569 false alarms on the Trace dataset, with an average only 40 false alarms every day. Security analysts can easily handle this number of alarms and do security investigations on them. If the two-stage detection described in Sec.~\ref{sec_overview_revised} is applied, the average number of false alarms every day can be further lowered to 24.}

We further note that neither \system{} nor other similar APT detection approaches are complete end-to-end detectors. The entire detection pipeline requires the involvement of security auditing softwares (or devices) and the help of security analysts for further investigations and attack story recovery. The function of APT detection approaches like \system{} is to reduce the workload of security experts and reduce the demand for human interference. An average 40 or 24 false alarms every day is more than acceptable in practice.

\vspace{0.5em}\noindent\textbf{MR14: Provide a more detailed run-time analysis on more parameters (Rev \#C).}\vspace{0.5em}

We have re-checked the run-time analysis attached to our previous versions and revised it to include more parameters such as $t$, $d$, $l$, $r$ and $k$ in Appendix~\ref{appe_b_revised}.

\textcolor{blue}{Given number of system entities $N$, number of system interactions $E$, initial embedding dimension \emph{t}, graph representation dimension $d$, number of GAT layers $l$ and mask rate $r$ the graph construction steps builds a featured provenance graph in $O((N+E) * t)$ time, masked feature reconstruction is completed in $O((N+E) * d^2 * l * r)$ time and sample-based structure reconstruction takes only $O(N * d)$ time. Training of the detection module takes $O(N *logN * d)$ time to build a K-D Tree and memorize benign embeddings. Detection result of a single target is obtained in $O(logN * d * k)$ time. Thus, the overall time complexity of \system{} during training and inference is $O(N*logN * d * k+E * d ^2 * l * r + (N + E) * t)$.}

\textcolor{blue}{\system{}'s memory consumption largely depends on $d$ and $t$. The graph representation module takes up $O((N+E)*t)$ space to store a provenance graph and $O((N+E)*(t +d))$ space to generate output embeddings. The detection module takes $O(N*d)$ space to memorize benign embeddings. The overall space complexity of \system{} is $O((N+E)*(t+d))$.}

\vspace{0.5em}\noindent\textbf{MR15: Compare both the result and run-time overhead of MAGIC and ShadeWatcher on the same split (Rev \#D).}\vspace{0.5em}

During our redone experiments, we have changed our train ratio and aligned with ShadeWatcher. The experimental results, including \system{}'s effectiveness and its training and inference time on the DARPA E3 Trace is obtained under a train ratio of 80\%. Regarding the comparison of efficiency between \system{} and ShadeWatcher, we note that \textcolor{blue}{Compared with ShadeWatcher, \system{} is 51 times faster in training under the same train ratio setting (i.e. 80\% log entries for training on DARPA Trace dataset).}

\vspace{0.5em}\noindent\textbf{MR16: Clarify the figures in the individual component analysis to demonstrate how they affect \system{}'s performance and efficiency (Rev \#D).}\vspace{0.5em}

Concerning the individual component analysis, we have presented a new Figure~\ref{fig_ablation_revised_letter} to demonstrate how different reconstruction components affect \system{}'s effectiveness and efficiency and updated the individual component analysis sub-section.

\textcolor{blue}{\noindent\textbf{Individual Component Analysis.} We study how feature reconstruction (FR) as well as structure reconstruction (SR) affect \system{}'s performance and Figure~\ref{fig_ablation_revised} presents the impact of these component to both detection result and performance overhead. Both FR and SR provide supervision for \system{}'s graph representation module. Compared with ordinary FR, Masked FR slightly boosts performance and significantly reduces training time. Sampled-based SR, however, is an effective complexity reduction component which accelerates training without losing performance, compared with full SR.}

\begin{figure}[t]
    \centering
    \subfigure[FR, on Wget dataset]{\includegraphics[width=0.495\hsize]{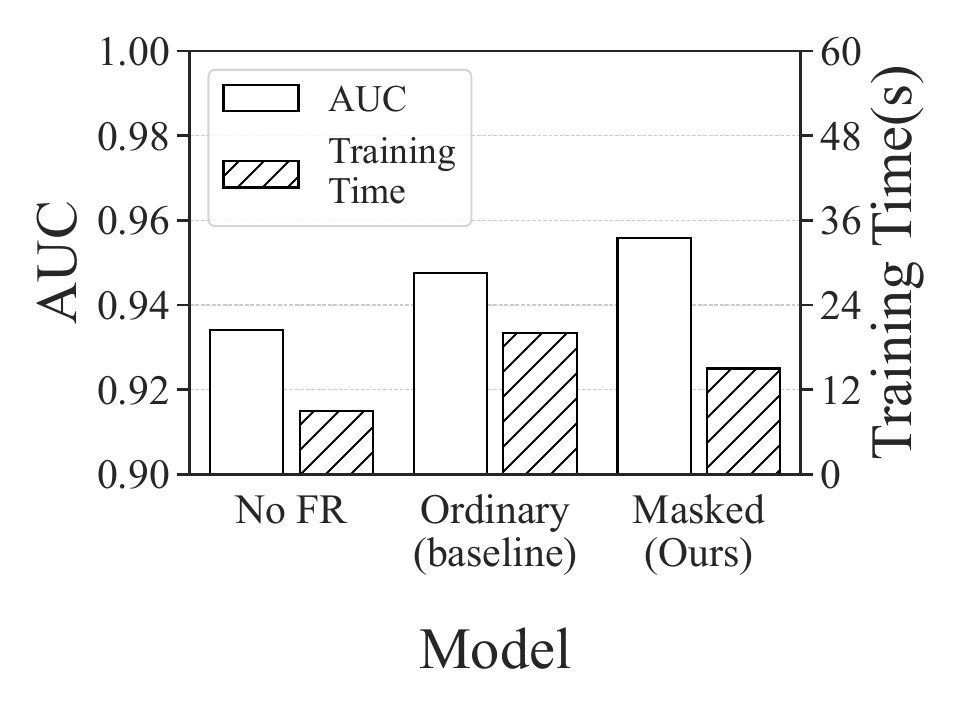}\label{fig_ablation_fr_letter}}
    \subfigure[SR, on Wget dataset]{\includegraphics[width=0.495\hsize]{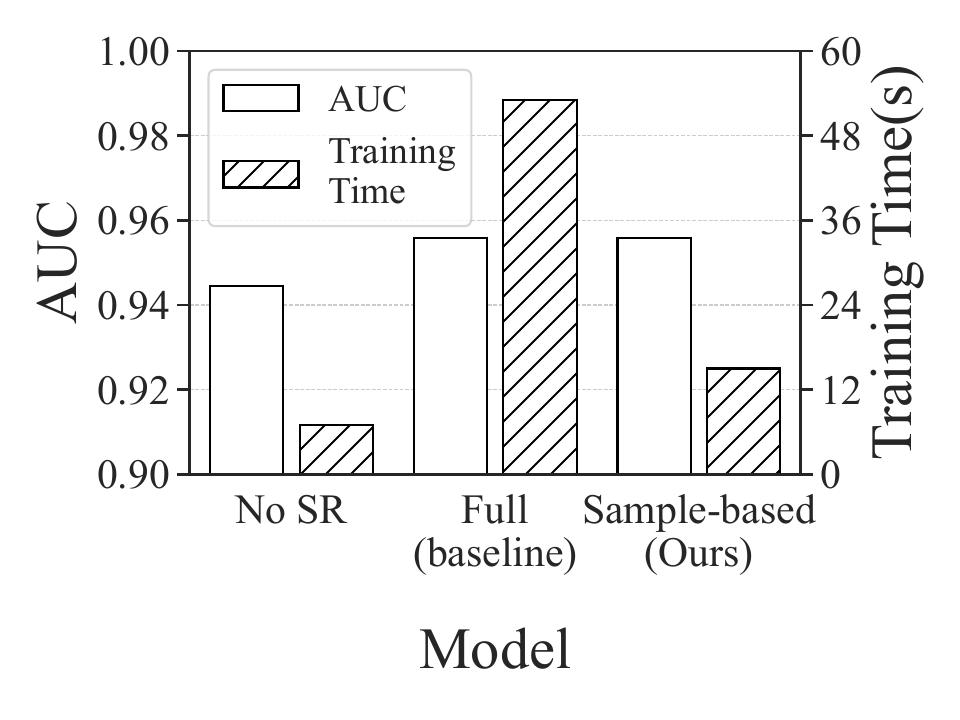}\label{fig_ablation_sr_letter}}
    \caption{Effect of different reconstruction components on \system{}'s performance and efficiency.}
    \label{fig_ablation_revised_letter}
\end{figure}
\vspace{0.5em}\noindent\textbf{MR17: Re-check the motivation examples and explain the portscan operation between \emph{tcexec} and the attacker (Rev \#D).}\vspace{0.5em}

There is no such operation between \emph{tcexec} and the attacker's IP address. We made a mistake and we have renewed the motivation example (Figure~\ref{fig_motivation_revised_letter}) to address its correctness. The case study uses the same example and has been consequently changed (Figure~\ref{fig_case_revised_letter}).

\vspace{0.5em}\noindent\textbf{MR18: Include precision metric into \system{}'s evaluation (Rev \#E).}\vspace{0.5em}

We have added precision as well as AUC as two of our evaluation metrics, especially in the comparison study in Sec.~\ref{sec_evaluation_2_revised}. We again present the result in Table~\ref{tab_compare_result_revised_letter}. 

\begin{table}[t]
\setlength{\abovecaptionskip}{0cm}
\setlength{\belowcaptionskip}{0.2cm}
\caption{Comparison between \system{} and state-of-the-art APT detection methods on different datasets. Within column \emph{supervision}, B indicates benign data, A refers to attack data and SA for streaming attack data.}
\label{tab_compare_result_revised_letter}

\resizebox{\columnwidth}{!}{
\begin{tabular}{|c|c|c|c|c|c|c|c|}

\hline
Dataset & Approach & Train Ratio & Supervision & Precision &  F1-Score & Recall & FPR\\
\hline\hline

\multirow{5}{*}{StreamSpot} & StreamSpot & 80\% & B & 73\% & 81\% & 91\% & 6.6\%\\

 & Unicorn (baseline) & 75\% & B & 95\% & 96\% & 93\% & 1.6\%\\

 & Prov-Gem & 80\% & B,A & 100\% & 97\% & 94\% & \textbf{0\%}\\

 & ThreaTrace & 75\% & B & 98\% & 99\% & 99\% & 0.4\%\\

 & \textbf{\system{} (Ours)} & 80\% & B & 99\% & \textbf{99\%} & \textbf{100\%} & 0.6\%\\
\hline\hline

\multirow{4}{*}{\makecell[c]{Unicorn\\Wget}} & Unicorn (baseline) & 80\% & B & 86\% & 90\% & 95\% & 15.5\%\\

 & Prov-Gem & 80\% & B,A & 100\% & 89\% & 80\% & \textbf{0\%}\\

 & ThreaTrace & 80\% & B & 93\% & 95\% & \textbf{98\%} & 7.4\%\\

 & \textbf{\system{} (Ours)} & 80\% & B & 98\% & \textbf{97\%} & 96\% & 2.0\%\\
\hline\hline

\multirow{5}{*}{\makecell[c]{DARPA\\E3 Trace}} & DeepLog & N/A & B,A & 41\% & 51\% & 68\% & 2.7\%\\

& Log2vec (baseline) & N/A & B,A & 54\% & 64\% & 78\% & 1.8\%\\

& ThreaTrace & N/A & B & 72\% & 83\% & 99\% & 1.1\%\\

& ShadeWatcher & 80\% & B,SA & 97\% & 99\% & \textbf{99\%} & 0.3\%\\

 & \textbf{\system{} (Ours)} & 80\% & B & \textbf{99\%} & \textbf{99\%} & 99\% &\textbf{0.1\%}\\
\hline\hline

\multirow{4}{*}{\makecell[c]{DARPA\\E3 THEIA}} & DeepLog & N/A & B,A & 16\% & 15\% & 14\% & 0.5\%\\

& Log2vec (baseline) & N/A & B,A & 62\% & 64\% & 66\% & 0.3\%\\

& ThreaTrace & N/A & B & 87\% & 93\% & 99\% & \textbf{0.1\%}\\

 & \textbf{\system{} (Ours)} & 80\% & B & \textbf{98\%} & \textbf{99\%} & \textbf{99\%} & 0.1\%\\
\hline\hline

\multirow{4}{*}{\makecell[c]{DARPA\\E3 CADETS}} & DeepLog & N/A & B,A & 23\% & 35\% & 74\% & 4.4\%\\

& Log2vec (baseline) & N/A & B,A & 49\% & 62\% & 85\% & 1.6\%\\

& ThreaTrace & N/A & B & 90\% & 95\% & \textbf{99\%} & 0.2\%\\

 & \textbf{\system{} (Ours)} & 80\% & B & \textbf{94\%} & \textbf{97\%} & 99\% & \textbf{0.2\%}\\
\hline
\end{tabular}
}
\end{table}

\vspace{0.5em}\noindent\textbf{MR19: Provide per-attack results for experiments (Rev \#A).}\vspace{0.5em}

We have reported per-attack detection results in Table~\ref{tab_general_result_revised_letter}, which is included in \textbf{MR1}. We also note that among the four attack scenarios mentioned in the DARPA E3 ground truth document, the three attack strategies \emph{Extension Backdoor}, \emph{Phishing Executable} and \emph{Pine Backdoor} forms a successful attack attempt. The \emph{Firefox Backdoor} attack is a failure and is not related to the other three attacks. To align with ThreaTrace~\cite{aptlearnbasedthreatrace-17}, we have removed \emph{Firefox Backdoor} and all the interactions related to it from the raw logs.

\vspace{0.5em}\noindent\textbf{MR20: Try to search for \system{}'s disadvantages in entity level detection (Rev \#A).}\vspace{0.5em}

We have analyzed the per-entity detection result of \system{} on DARPA E3 Trace dataset and we have found a weakness. As stated in Sec.~\ref{sec_evaluation_2_revised}, \textcolor{blue}{Among the false negative results, we notice that most of them are malicious files and libraries involved in the attacks. This indicates that \system{} excels at detecting malicious processes and network connections that behaves differently from benign system entities. However, \system{} finds it hard to locate passive entities such as malicious files and libraries, whose behaviors tend to be similar to benign ones. Fortunately, these intermediate files and libraries can be easily identified during attack story recovery, given the malicious processes and connections successfully detected.} Additionally, the adversarial attack experiments mentioned in \textbf{MR3} reveals that \system{} is less robust against Benign Feature Poison attacks, which have caused a drop in \system{}'s AUC. These stand for the disadvantages of \system{} in entity level detection we have found so far.

~\\\\
 \textbf{For other comments in rebuttal, including “relationship with anomaly detection”, “ground truth label for entity level datasets” and other minor yet constructive comments, we would like to refer the reviewers to our earlier responses in the MR items for more details. Thanks!}
